# Supplementary material for: Synthetic Wavelength Holography: An Extension of Gabor's Holographic Principle to Imaging with Scattered Wavefronts
Source: arXiv:1912.11438 ancillary file (2020-11-23)
Supplement: Supplementary file 1 [file SupplementaryMaterial__Willomitzer_SWH.pdf]

# Supplementary material for manuscript "An extension of Gabor's Holographic Principle to Imaging with Scattered Wavefronts"

## *Introduction*

It is common knowledge in holography and interferometry that peak-to-valley excursions in the wavefront error (wave aberration) that are limited to ¼ of the optical wavelength (Rayleigh criterion) introduce minimal errors in the retrieved intensity and phase of an optical field. However, it is not apparent that computational mixing of scattered fields recorded at two closely spaced wavelengths $\lambda_1, \lambda_2$, each of which exhibits wavefront aberrations far in excess of ¼ of the optical wavelength, do indeed preserve phase information at scales smaller than the synthetic wavelength $\Lambda = \frac{|\lambda_1 - \lambda_2|}{\lambda_1 \lambda_2}$. The present document puts forth a mathematical basis for the aforementioned claim. The analysis accommodates scattering at optically rough surfaces, optical blurring in an imaging optic and sampling at the detector. The analysis while broad in scope, focuses on the application of imaging objects that are beyond the imager line-of-sight (LoS) and obscured from view. The canonical scene arrangement of **Figure1** is used to introduce relevant concepts.

Our approach exploits the availability of an intermediary scattering surface (such as the wall in **Figure1**) in

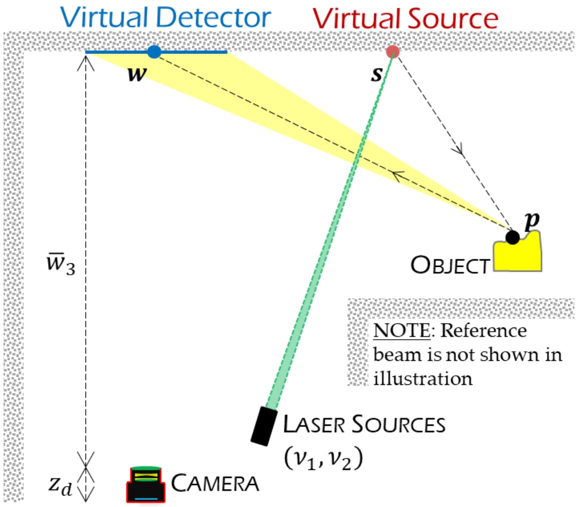


**Figure1:** Canonical Scene arrangement for indirect imaging of objects obscured from view

serving the dual purpose of illuminating objects obscured from view and intercepting the light scattered by the obscured objects. Accordingly, the intermediary surface may be viewed as a virtualized source of illumination and detection for the obscured objects. Herein, we seek to simultaneously recover a spatially resolved image of the obscured objects and their position within the hidden volume. To this end, we record the optical field emerging from the intermediary surface, using a holographic imaging apparatus (camera in **Figure1**). The recorded hologram, however, bears little resemblance to the macroscopic structure of the obscured object, due in large part to the randomzied dephasing of light following a reflection at the intermediary surface. Circumventing this problem without any knowledge of the scattering properties of the intermediary surface is a key contribution of our work. It is made possible by interrogating the hidden scene using two closely spaced optical frequencies and exploiting the spectral correlation in scattering at the intermediary surface.

The notion of exploiting spectral correlations in mitigating the deleterious effects of randomzied dephasing due to repeated scattering, has broad applications ranging from imaging through scattering/turbid media, imaging through tissue, imaging through fog/smoke, and imaging under brownout conditions. This document describes the mathematical principles underpinning the use of spectral field correlations in adapting scattering as degree of freedom from the standpoint of imaging.

In the interest of clarity, attention is restricted to the modeling the propagation of coherent light in the canonical scene of **Figure1**, and the subsequent recovery of a hologram of the obscured object(s). The task of accurately modeling light propagation within the canonical scene is exceedingly difficult, due in large part to the multiplicity of scattering surfaces and numerous light bounces. The task is further complicated by factors such as multiple scattering at interfaces, shadowing, and Fresnel reflections. Incorporating these effects into a comprehensive model for imaging is mathematically intractable. Imposing specific restrictions and simlyfing assumptions allows us to develop a mathematically tractable framework for light transport in the canonical scene. The list of restrictions and simplifying assumtions are enumerated below:

1. A linearly polarized narrow-linewidth tunable CW laser source with center frequency $\bar{\nu}$ is used to interrogate the hidden scene by illuminating the Virtual Souce surface.
2. Scalar diffraction is sufficient to model field transport through the scene.
3. The temporal fluctuations of the CW laser source are statistically uncorrelated with those of ambient light sources in the scene.
4. The principal contribution to the irradiance observed at the sensor is restricted to three bounce ray paths originating at the physical source, bouncing off the Virtual Source surface, the hidden object and the Virtual Detector surface, prior to terminating at the physical detector. The radiometric throughput of fourth and higher order bounces is assumed to be negligibly small, a fact borne out in experiments.
5. The coherence length of the source exceeds the cumulative length of all three-bounce ray originating at the physical source, traversing the hidden scene and terminating at the physical sensor. Consequently, the indirectly illuminated object can be expressed as a countably-finite collection of secondary point sources that are mutually coherent.
6. The propagation medium is free space and devoid of inhomogenities. The propagation distances exceed the spatial extent of the Virtual Source and the Virtual Detector.
7. Physical objects in the scene are optically rough at the scale of the optical wavelength of the CW laser source. We assume that path length variations induced by fluctuations in the surface height are the sole source of scattering, consistent with Goodman's approach [1].
8. A diffraction limited optic is used to relay the image of the Virtual Detector surface onto an image sensor. The coordinate system used to develop the model is centered about entrance pupil of the imaging optic, $XY$ plane is aligned with image sensor and $Z$-axis is aligned with the optical axis
9. A lock-in sensor whose operation is described in [2], records interference of light scattered by obscured object and a planar reference beam. The lock-In camera (Lock-In sensor + imaging optics) independently acquires holograms of coherently illuminated scene/object
10. The reference beam envelope and phase does not change appreciably over the finite extent of a single detector pixel.

11. The illumination source subtends a small solid angle with respect to the obscured object. The spectral reflectance of source is unchanged for small change in optical frequency of illumination source.

12. The object albedo is unchanged for small change in optical frequency of illumination source

13. The defocus error introduced by the microscopic roughness of the Virtual Detector surface is negligible.

### *Key findings/claims*

1. A small change $\Delta\nu$ in the optical frequency of the CW source used to interrogate the hidden scene of **Figure1** imparts an additional spherical phase component to the field contribution of each obscured object point. The excess spherical phase encodes the position of the obscured object at the "synthetic" wavelength $c\Delta\nu^{-1}$ meters. **(Eqs.(28),(29))**
2. Computational mixing of holograms recorded at two closely spaced optical frequencies encapsulates field information at sub-millimeter synthetic wavelength scales that are insensitive to scattering at the optical frequency of interrogation. **(Sections.1.5,1.6)**
3. Wavefront errors in the computational hologram are negligible if the change in optical path length stemming from a change $\Delta\nu$ in the optical frequency of interrogation is limited to $\frac{1}{4^{\text{th}}}$ synthetic wavelength $c\Delta\nu^{-1}$ meters, for any ray path originating at the source and terminating at the sensor. **(Section.1.6)**
4. Optical holograms acquired at regularly spaced optical frequencies may be combined to computationally filter light paths with a prescribed round-trip distance from the physical source to the physical detector, so long as condition-3 holds for the largest frequency separation. **(Section.2)**

### *Notation*

The mathematical analysis furnished in this document oftentimes involves multiple integrals and summations over spatial and time dimensions that can be continuous or discrete. In an effort to improve the clarity of the analysis we adopt the following convention in describing quantities of interest.

| | | | |
|---|---|---|---|
| $\boldsymbol{x}$ | Position vector of a point on the sensor plane | $\in \mathbb{R}^2$ | meters |
| $\boldsymbol{d}$ | Position vector associated with a point on the Virtual Detector | $\in \mathbb{R}^3$ | meters |
| $\boldsymbol{s}$ | Position vector associated with a point on the Virtual Source | $\in \mathbb{R}^3$ | meters |
| $\boldsymbol{p}$ | Position vector associated with the obscured object point | $\in \mathbb{R}^3$ | meters |
| $\bar{\nu}$ | Optical frequency of the CW source used to interrogate the hidden scene | | THz |
| $\bar{\omega} = 2\pi\bar{\nu}$ | Angular frequency of the CW source used to interrogate the hidden scene | | radians |
| $t$ | Time | | seconds |
| $I$ | Irradiance (real valued & non-negative) | $\in \mathbb{R}^{2+}$ | arbitrary units |
| $\mathcal{U}$ | Optical field (complex-valued) | $\in \mathbb{C}^2$ | arbitrary units |
| $\Delta$ | Sensor pixel pitch (in $\mu m$) | | Microns |
| $F$ | Fill factor of sensor pixel ($0 < F \leq 1$) | $\in \mathbb{R}^+$ | dimensionless |

## *Key expressions*

Key expressions from the mathematical analysis are summarized in **Figure2**. These include the expression for the sampled holograms at two closely optical frequencies, and a mathematical formulation of Claim-1.

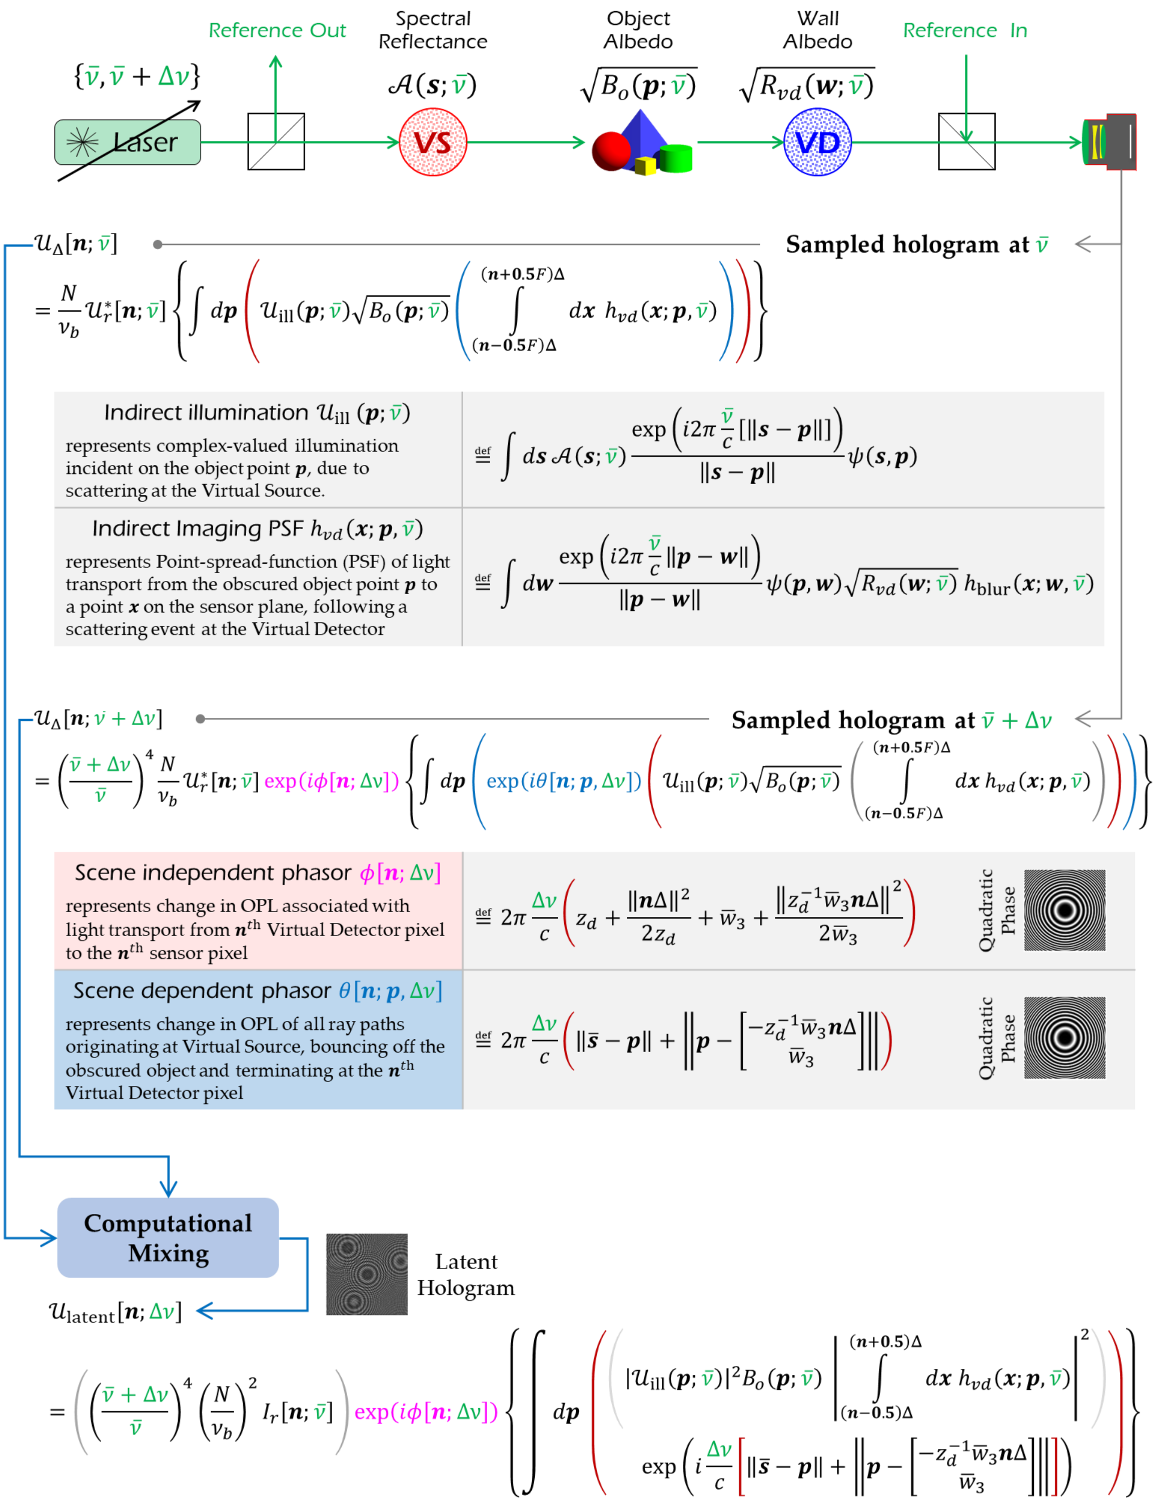


**Figure2:** Key mathematical expressions

In the interest of clarity, the task of modeling light transport in the canonical scene of **Figure1** is sub-divided into two tasks. The first of these tasks seeks to model the process of imaging the Virtual Detector surface including sampling at the image sensor. The second task models the physical propagation of light originating at the Virtual Source, bouncing off the obscured object and terminating at the Virtual Detector.

## *1.1 Imaging identity and optical blur*

Without loss of generality, it is assumed that light emerging from the Virtual Detector surface is relayed to the Lock-In sensor using a well-corrected optic with focal length $f$ and unity pupil magnification. The relation between a point on the Virtual Detector surface and its pixel projection on the image sensor satisfies the following geometric relation:

$$x_1 = -z_d \frac{w_1}{w_3} \quad , \; x_2 = -z_d \frac{w_2}{w_3} \tag{1}$$

The term $z_d$ represents the distance from the sensor plane to the exit pupil plane of the imaging optics. The negative sign accommodates image inversion. If the imager optical axis and the macroscopic normal vector to the Virtual Detector surface (disregarding change in local surface normal due to microscopic roughness of VD surface) are aligned, then the magnification $z_d^{-1} w_3 \approx z_d^{-1} \bar{w}_3$, where $\bar{w}_3$ is the macroscopic perpendicular distance from the VD surface to the entrance pupil plane of the imaging optics.

The diffraction limited optical blur associated with imaging the VD surface may be modeled as a paraxial blur [3] with image side numerical aperture $D z_d^{-1}$, where $D$ is the diameter of the exit pupil. The resulting amplitude PSF is disclosed in Eq.(2). The term $P(u, v)$ represents the transmittance function of the exit pupil and modeled as an indicator function with diameter $D$. The term $f$ represents the focal length of the imaging optic. The depth $w_3$ of a point on the VD surface is measured with respect to the entrance pupil plane of the imaging optic.

$$\mathrm{h_{blur}}\left(\boldsymbol{x} \stackrel{\text{def}}{=} \begin{bmatrix} x_1 \\ x_2 \end{bmatrix}; \boldsymbol{w} \stackrel{\text{def}}{=} \begin{bmatrix} w_1 \\ w_2 \\ w_3 \end{bmatrix}, \bar{\nu}\right) = \left( \begin{matrix} \left(\frac{\bar{\nu}}{ic}\right)^2 \frac{1}{z_d w_3} \exp\left(i \frac{2\pi\bar{\nu}}{c}\left[z_d + w_3 + \frac{[x_1^2 + x_2^2]}{2z_d} + \frac{[w_1^2 + w_2^2]}{2w_3}\right]\right) \times \\ \int dudv \left(P(u,v) \exp\left(i \frac{2\pi\bar{\nu}}{c}\left[\frac{1}{z_d} + \frac{1}{w_3} - \frac{1}{f}\right](u^2 + v^2)\right) \exp\left(-i \frac{2\pi\bar{\nu}}{c}\left(\left[\frac{x_1}{z_d} + \frac{w_1}{w_3}\right] u + \left[\frac{x_2}{z_d} + \frac{w_2}{w_3}\right] v\right)\right)\right) \end{matrix} \right) \tag{2}$$

## *1.2 Recording optical fields using the Lock-In sensor*

As is common practice in holography and interferometry, we acquire optical fields by recording the interference of the said field with a reference beam whose temporal fluctuations are highly correlated with the desired optical field. To this end, the field incident on the Lock-In sensor may be expressed as the superposition of the field contributions from the indirectly illuminated object and a planar reference beam, as shown below:

$$\mathcal{U}(\boldsymbol{x}, t; \bar{\nu}) = \mathcal{U}_o(\boldsymbol{x}; \bar{\nu}) \exp(i\bar{\omega}t) + \mathcal{U}_r(\boldsymbol{x}; \bar{\nu}) \exp(i[\bar{\omega} + \omega_b]t) \tag{3}$$

The term $\mathcal{U}_r(\boldsymbol{x}; \bar{\nu})$ in Eq.(3) represents the baseband envelope of the reference field incident on the Lock-in sensor plane. The term $\mathcal{U}_o(\boldsymbol{x}; \bar{\nu})$ represents the baseband envelope of the subjective speckle field due to the indirectly illuminated object/target. The angular frequency difference $\omega_b$ between the two arms of the interferometer helps in isolating the desired field component from the corrupting influence of the zeroth

order and twin components that arise during square-law detection of the irradiance $|\mathcal{U}(\boldsymbol{x},t;\bar{\nu})|^2$. Insight into the process can be gleaned by examining the expression for the instantaneous irradiance incident on the Lock-In sensor plane, disclosed in Eq.(4).

$$\begin{aligned} I(\boldsymbol{x},t;\bar{\nu}) &= |\mathcal{U}(\boldsymbol{x},t;\bar{\nu})|^2 \\ &= |\mathcal{U}_o(\boldsymbol{x};\bar{\nu})|^2 + |\mathcal{U}_r(\boldsymbol{x};\bar{\nu})|^2 + 2\,\mathcal{R}eal\{\mathcal{U}_o(\boldsymbol{x};\bar{\nu})\mathcal{U}_r^*(\boldsymbol{x};\bar{\nu})\exp(-i\omega_b t)\} \\ &= |\mathcal{U}_o(\boldsymbol{x};\bar{\nu})|^2 + |\mathcal{U}_r(\boldsymbol{x};\bar{\nu})|^2 + 2|\mathcal{U}_o(\boldsymbol{x};\bar{\nu})| \times |\mathcal{U}_r(\boldsymbol{x};\bar{\nu})|\cos(\varphi_o(\boldsymbol{x};\bar{\nu}) - \varphi_r(\boldsymbol{x};\bar{\nu}) - \omega_b t) \\ &= I_o(\boldsymbol{x};\bar{\nu}) + I_r(\boldsymbol{x};\bar{\nu}) + 2\sqrt{I_o(\boldsymbol{x};\bar{\nu})}\sqrt{I_r(\boldsymbol{x};\bar{\nu})}\cos(\varphi_o(\boldsymbol{x};\bar{\nu}) - \varphi_r(\boldsymbol{x};\bar{\nu}) - \omega_b t) \end{aligned} \quad (4)$$

The instantaneous intensity recorded by the $\boldsymbol{n}^{th}$ Lock-In pixel is obtained by integrating the irradiance $I(\boldsymbol{x},t;\bar{\nu})$ incident on its active area. The corresponding expression is disclosed below:

$$\begin{aligned} I[\boldsymbol{n},t;\bar{\nu}] &= \int_{(\boldsymbol{n}-0.5F)\Delta}^{(\boldsymbol{n}+0.5F)\Delta} d\boldsymbol{x}\, I(\boldsymbol{x},t;\bar{\nu}) \\ &= \left\{\int_{(\boldsymbol{n}-0.5F)\Delta}^{(\boldsymbol{n}+0.5F)\Delta} d\boldsymbol{x}\,[I_o(\boldsymbol{x};\bar{\nu}) + I_r(\boldsymbol{x};\bar{\nu})]\right\} + \left\{2\int_{(\boldsymbol{n}-0.5F)\Delta}^{(\boldsymbol{n}+0.5F)\Delta} d\boldsymbol{x}\left[\sqrt{I_o(\boldsymbol{x};\bar{\nu})}\sqrt{I_r(\boldsymbol{x};\bar{\nu})}\cos(\varphi_o(\boldsymbol{x};\bar{\nu}) - \varphi_r(\boldsymbol{x};\bar{\nu}) - \omega_b t)\right]\right\} \end{aligned} \quad (5)$$

Following assumption-6, the envelope and phase of the reference beam does not change appreciably over the finite extent of a single detector pixel, so that:

$$\left.\begin{aligned} I_r(\boldsymbol{x};\bar{\nu}) \approx I_r(\boldsymbol{n}\Delta;\bar{\nu}) \stackrel{\text{def}}{=} I_r[\boldsymbol{n};\bar{\nu}] \\ \cos(\varphi_r(\boldsymbol{x};\bar{\nu})) \approx \cos(\varphi_r(\boldsymbol{n}\Delta;\bar{\nu})) \stackrel{\text{def}}{=} \cos(\varphi_r[\boldsymbol{n};\bar{\nu}]) \end{aligned}\right\} \quad \forall\, \boldsymbol{x} \in (\boldsymbol{n}\Delta - \mathbf{0.5}F\Delta, \boldsymbol{n}\Delta + \mathbf{0.5}F\Delta) \quad (6)$$

As a result, the reference beam's contribution to the integrated irradiance may be simplified as follows:

$$\left\{\int_{(\boldsymbol{n}-0.5F)\Delta}^{(\boldsymbol{n}+0.5F)\Delta} d\boldsymbol{x}\, I_r(\boldsymbol{x};\bar{\nu})\right\} \approx \left\{\int_{(\boldsymbol{n}-0.5F)\Delta}^{(\boldsymbol{n}+0.5F)\Delta} d\boldsymbol{x}\, I_r(\boldsymbol{n}\Delta;\bar{\nu})\right\} \approx I_r[\boldsymbol{n};\bar{\nu}]\left\{\int_{(\boldsymbol{n}-0.5F)\Delta}^{(\boldsymbol{n}+0.5F)\Delta} d\boldsymbol{x}\right\} \approx \Delta^2 \times I_r[\boldsymbol{n};\bar{\nu}] \quad (7)$$

Incorporating Eqs.(7) & (6) into Eq.(5) yields the following expression for the instantaneous irradiance recorded by the $\boldsymbol{n}^{th}$ lock-in pixel:

$$\begin{aligned} &I[\boldsymbol{n},t;\bar{\nu}] \\ &\approx \left\{\Delta^2 \times I_r(\boldsymbol{n}\Delta;\bar{\nu}) + \int_{(\boldsymbol{n}-0.5F)\Delta}^{(\boldsymbol{n}+0.5F)\Delta} d\boldsymbol{x}\,[I_o(\boldsymbol{x};\bar{\nu})]\right\} + \left\{2\sqrt{I_r[\boldsymbol{n};\bar{\nu}]}\int_{(\boldsymbol{n}-0.5F)\Delta}^{(\boldsymbol{n}+0.5F)\Delta} d\boldsymbol{x}\left[\sqrt{I_o(\boldsymbol{x};\bar{\nu})}\cos(\varphi_o(\boldsymbol{x};\bar{\nu}) - \varphi_r[\boldsymbol{n};\bar{\nu}] - \omega_b t)\right]\right\} \\ &\approx \left(\begin{aligned} &\left\{\Delta^2 \times I_r[\boldsymbol{n};\bar{\nu}] + \left[\int_{(\boldsymbol{n}-0.5F)\Delta}^{(\boldsymbol{n}+0.5F)\Delta} d\boldsymbol{x}\, I_o(\boldsymbol{x};\bar{\nu})\right]\right\} + \left\{2\sqrt{I_r[\boldsymbol{n};\bar{\nu}]}\cos(\omega_b t)\left[\int_{(\boldsymbol{n}-0.5F)\Delta}^{(\boldsymbol{n}+0.5F)\Delta} d\boldsymbol{x}\left[\sqrt{I_o(\boldsymbol{x};\bar{\nu})}\cos(\varphi_o(\boldsymbol{x};\bar{\nu}) - \varphi_r[\boldsymbol{n};\bar{\nu}])\right]\right]\right\} \\ &+ \left\{2\sqrt{I_r[\boldsymbol{n};\bar{\nu}]}\sin(\omega_b t)\left[\int_{(\boldsymbol{n}-0.5F)\Delta}^{(\boldsymbol{n}+0.5F)\Delta} d\boldsymbol{x}\left[\sqrt{I_o(\boldsymbol{x};\bar{\nu})}\sin(\varphi_o(\boldsymbol{x};\bar{\nu}) - \varphi_r[\boldsymbol{n};\bar{\nu}])\right]\right]\right\} \end{aligned}\right) \end{aligned} \quad (8)$$

The first term in Eq.(8) represents the zeroth-order time-invariant irradiance contribution of the hologram recorded at $\bar{\nu}$. The second and third terms in Eq.(8) represents the time-varying irradiance contribution associated with the detector integration of the real & imaginary part of the subjective speckle field $\mathcal{U}_o(\boldsymbol{x};\bar{\nu})$, respecively. The temporal carrier associated with these terms has angular frequency $\omega_b$ and phase $\frac{\pi}{2} - \varphi_r[\boldsymbol{n};\bar{\nu}]$ and $-\varphi_r[\boldsymbol{n};\bar{\nu}]$ respectively. The amplitude $\sqrt{I_r[\boldsymbol{n};\bar{\nu}]}$ of these terms describes the heterodyne gain arising from synchronous demodulation at $\omega_b$. The integral over spatial locations in the second and third terms signify the real and imaginary parts of the phasor sum of the subjective speckle cells that can be accommodated within the $\boldsymbol{n}^{th}$ detector pixel. The integration accommodates signal fading arising from the summation of a disproportionately large number of statistically independent speckle cells [4].

Each pixel of the Lock-in sensor functions as a homodyne reciever that accumlates the result of demodulating the received irradiance with two local oscillator (LO) signals $\sin(\omega_b t)$ and $\cos(\omega_b t)$ that are in quadrature phase. The demodulation is restricted to $N$ periods of the LO signal, and yields a sampled representation of the in-phase (real part) & quadrature (imaginary part) components of the complex-valued optical field incident on the Lock-In sensor. The expression for the in-phase component of the optical field recorded by the Lock-In sensor is furnished below:

$$I_I[\boldsymbol{n};\bar{\nu}] = \int_{t=0}^{N\nu_b^{-1}} dt \cos(\omega_b t)\, I[\boldsymbol{n},t;\bar{\nu}]$$

$$= \left\{\int_{t=0}^{N\nu_b^{-1}} dt\, cos(\omega_b t)\, cos(\omega_b t)\right\}\left\{2\sqrt{I_r[\boldsymbol{n};\bar{\nu}]}\int_{(\boldsymbol{n}-0.5F)\Delta}^{(\boldsymbol{n}+0.5F)\Delta} d\boldsymbol{x}\left[\sqrt{I_o(\boldsymbol{x};\bar{\nu})}\cos(\varphi_o(\boldsymbol{x};\bar{\nu}) - \varphi_r[\boldsymbol{n};\bar{\nu}])\right]\right\}$$

$$= \left\{\frac{1}{2}\int_{t=0}^{N\nu_b^{-1}} dt[1 + cos(2\omega_b t)]\right\}\left\{2\sqrt{I_r[\boldsymbol{n};\bar{\nu}]}\int_{(\boldsymbol{n}-0.5F)\Delta}^{(\boldsymbol{n}+0.5F)\Delta} d\boldsymbol{x}\left[\sqrt{I_o(\boldsymbol{x};\bar{\nu})}\cos(\varphi_o(\boldsymbol{x};\bar{\nu}) - \varphi_r[\boldsymbol{n};\bar{\nu}])\right]\right\}$$

$$= N\nu_b^{-1}\sqrt{I_r[\boldsymbol{n};\bar{\nu}]}\left\{\int_{(\boldsymbol{n}-0.5F)\Delta}^{(\boldsymbol{n}+0.5F)\Delta} d\boldsymbol{x}\left[\sqrt{I_o(\boldsymbol{x};\bar{\nu})}\cos(\varphi_o(\boldsymbol{x};\bar{\nu}) - \varphi_r[\boldsymbol{n};\bar{\nu}])\right]\right\} \qquad (9)$$

The expression for the quadrature component of the optical field recorded by the Lock-In sensor is furnished below:

$$I_Q[\boldsymbol{n};\bar{\nu}] = \int_{t=0}^{N\nu_b^{-1}} dt \sin(\omega_b t)\, I[\boldsymbol{n},t;\bar{\nu}]$$
$$= N\nu_b^{-1}\sqrt{I_r[\boldsymbol{n};\bar{\nu}]}\left\{\int_{(\boldsymbol{n}-0.5F)\Delta}^{(\boldsymbol{n}+0.5F)\Delta} d\boldsymbol{x}\left[\sqrt{I_o(\boldsymbol{x};\bar{\nu})}\sin(\varphi_o(\boldsymbol{x};\bar{\nu}) - \varphi_r[\boldsymbol{n};\bar{\nu}])\right]\right\} \qquad (10)$$

By combining the sampled in-phase and quadrature images, the sampled hologram at the optical wavelength may be reconstituted, as shown in Eq.(11).

$$\mathcal{U}_\Delta[\boldsymbol{n};\bar{\nu}] = I_I[\boldsymbol{n};\bar{\nu}] + \sqrt{-1}I_Q[\boldsymbol{n};\bar{\nu}]$$
$$= N\nu_b^{-1}\sqrt{I_r[\boldsymbol{n};\bar{\nu}]}\left\{\int_{(\boldsymbol{n}-0.5F)\Delta}^{(\boldsymbol{n}+0.5F)\Delta} d\boldsymbol{x}\left[\sqrt{I_o(\boldsymbol{x};\bar{\nu})}\exp\left(i[\varphi_o(\boldsymbol{x};\bar{\nu}) - \varphi_r[\boldsymbol{n};\bar{\nu}]]\right)\right]\right\}$$
$$= N\nu_b^{-1}\sqrt{I_r[\boldsymbol{n};\bar{\nu}]}\exp(-i\varphi_r[\boldsymbol{n};\bar{\nu}])\left\{\int_{(\boldsymbol{n}-0.5F)\Delta}^{(\boldsymbol{n}+0.5F)\Delta} d\boldsymbol{x}\left[\sqrt{I_o(\boldsymbol{x};\bar{\nu})}\exp\left(i\varphi_o(\boldsymbol{x};\bar{\nu})\right)\right]\right\} \qquad (11)$$
$$= N\nu_b^{-1}\mathcal{U}_r^*[\boldsymbol{n};\bar{\nu}]\left\{\int_{(\boldsymbol{n}-0.5F)\Delta}^{(\boldsymbol{n}+0.5F)\Delta} d\boldsymbol{x}\, \mathcal{U}_o(\boldsymbol{x};\bar{\nu})\right\}$$

We conclude our discussion on recording optical fields by enumerating the principal benefits of a Lock-In sensor, namely:

- The ability to detect a weak sinusoidal signal buried in strong background and noise (accommodate a wide range of ambient illumination levels)
- The heterodyne gain afforded by combination of background subtraction and synchronous demodulation of the received irradiance at each pixel (eliminates need for longer exposure times and optical stabilization of interferometer)
- Eliminating need for matching the optical power in the two interferometer arms
- Snapshot hologram acquisition with maximal utilization of the limited spatial bandwidth of the FPA, (no mechanical movement or temporal phase-shifting required for isolating the hologram term).

The interested reader is referred to [5],[6] for details on the mechanics of recoding holograms using heterodyne interferometry and the Lock-In sensor.

### *1.3 Light transport from the Virtual Source to the Virtual Detector*

The discussion in Sections-1.1,1.2 restricted attention to the process of recording optical fields. The present section is devoted to the development of a mathematical model for propagating quasi-monochromatic scalar optical fields in the canonical scene arrangement of **Figure1**.

Our analysis begins with the observation that light scattered by the Virtual Source surface behaves as a partially coherent source of illumination for the obscured objects. Each point on the indirectly illuminated object may then be viewed as a secondary source of partially coherent light that directs spherical wavefronts towards the Virtual Detector surface. Each of these spherical wavefronts is additionally scattered by the Virtual Detector surface before being intercepted by the finite collection aperture of the imaging optic. The resulting spatial pattern is recorded by the image sensor, and exhibits a mottled appearance reminiscent of speckle [1].

The combined field contribution of the obscured object is obtained as a weighted superposition of the elementary phasors associated with light paths originating at a point $\boldsymbol{s}$ on the Virtual Source, bouncing off an obscured object point $\boldsymbol{p}$, and terminating at the Virtual Detector point $\boldsymbol{w}$, whose geometric projection onto the image sensor is $\boldsymbol{x}$. The final expression for the obscured object field $\mathcal{U}_o(\boldsymbol{x};\bar{\nu})$ incident on the Lock-In sensor is disclosed below:

$$\begin{aligned}
&\mathcal{U}_o(\boldsymbol{x};\bar{\nu}) \\
&= \left(\frac{\bar{\nu}}{ic}\right)^2 \int d\boldsymbol{w} \int d\boldsymbol{p} \left( \left( \int d\boldsymbol{s}\, \mathcal{A}(\boldsymbol{s};\bar{\nu}) \frac{\exp\left(i2\pi\frac{\bar{\nu}}{c}\|\boldsymbol{s}-\boldsymbol{p}\|\right)}{\|\boldsymbol{s}-\boldsymbol{p}\|} \psi(\boldsymbol{s},\boldsymbol{p}) \right) \sqrt{B_o(\boldsymbol{p};\bar{\nu})} \frac{\exp\left(i2\pi\frac{\bar{\nu}}{c}\|\boldsymbol{p}-\boldsymbol{w}\|\right)}{\|\boldsymbol{p}-\boldsymbol{w}\|} \psi(\boldsymbol{p},\boldsymbol{w}) \right) \sqrt{R_{vd}(\boldsymbol{w};\bar{\nu})}\, h_{\text{blur}}(\boldsymbol{x};\boldsymbol{w},\bar{\nu}) \qquad (12) \\
&= \left(\frac{\bar{\nu}}{ic}\right)^2 \int d\boldsymbol{p} \left( \int d\boldsymbol{w} \left( \int d\boldsymbol{s}\, \mathcal{A}(\boldsymbol{s};\bar{\nu}) \sqrt{B_o(\boldsymbol{p};\bar{\nu})} \psi(\boldsymbol{s},\boldsymbol{p}) \psi(\boldsymbol{p},\boldsymbol{w}) \frac{\exp\left(i2\pi\frac{\bar{\nu}}{c}[\|\boldsymbol{s}-\boldsymbol{p}\|+\|\boldsymbol{p}-\boldsymbol{w}\|]\right)}{\|\boldsymbol{s}-\boldsymbol{p}\|\times\|\boldsymbol{p}-\boldsymbol{w}\|} \right) \sqrt{R_{vd}(\boldsymbol{w};\bar{\nu})}\, h_{\text{blur}}(\boldsymbol{x};\boldsymbol{w},\bar{\nu}) \right)
\end{aligned}$$

The innermost integral of Eq.(12) which is colored in magenta represents the complex-valued illumination incident on the obscured object point $\boldsymbol{p}$, following scattering at the Virtual source. It encapsulates light transport from the physical source to the obscured object point. The term $\mathcal{A}(\boldsymbol{s};\bar{\nu})$ represents the spectral reflectance of the Virtual Source. It represents the combined influence of the real-valued albedo of the Virtual Source surface, and the complex-valued illumination beam incident on the Virtual Source surface. The term $\sqrt{B_o(\boldsymbol{p};\bar{\nu})}$ represents the square-root of the real-valued albedo of the object point $\boldsymbol{p}$. It encapsulates reflection from an infinitesimally small area element $d\boldsymbol{p}$ in the immediate vicinity of the object point $\boldsymbol{p}$. The term $\sqrt{R_{vd}(\boldsymbol{w};\bar{\nu})}$ represents the square-root of the real-valued albedo of a point $\boldsymbol{w}$ on the Virtual Detector

surface. It encapsulates Lambertian reflection at the Virtual Detector surface. The term $h_{\text{blur}}$ represents the amplitude PSF of the imaging optic and encapsulates diffraction limited imaging under coherent illumination.

*Accommodating scattering*

The length of the ray paths $\|\boldsymbol{s}-\boldsymbol{p}\|$ encapsulate the microscopic roughness of the Virtual Source surface and the obscured object. The corresponding phase fluctuations given by $\frac{\bar{\nu}}{c}\|\boldsymbol{s}-\boldsymbol{p}\|$ induce randomized dephasing of the spherical waves arriving at the obscured object point, mainfesting as speckle illumination. In a similar fashion, the length of the ray paths $\|\boldsymbol{p}-\boldsymbol{w}\|$ encapsulate the microscopic roughness of the obscured object and the Virtual Detector surface. The corresponding phase fluctuations given by $2\pi\frac{\bar{\nu}}{c}\|\boldsymbol{p}-\boldsymbol{w}\|$ induce randomized dephasing in the spherical waves arriving at the Virtual Detector surface, irreversibly corrupting the phase of the obscured object field propagting towards the Virtual Detector surface. Phase fluctuations arising from scattering at the object are embedded in the path length calculations $\|\boldsymbol{s}-\boldsymbol{p}\|$, $\|\boldsymbol{p}-\boldsymbol{w}\|$.

*Connection to conventional imaging*

By decoupling ray paths from the Virtual Source → obscured object → Virtual Detector into its constituent paths namely: Virtual Source → obscured object, and obscured object → Virtual Detector, it is posssible to recast the expression for the object field contribution at the Lock-In sensor in a mathematical form that closely resembles the standard space-variant imaging formulation [7]. In particular, the field contribution of the obscured object may be expressed as a coherent superposition of stochastic patterns that are each weighted by the real-valued albedo of the obscured object:

$$\mathcal{U}_o(\boldsymbol{x};\bar{\nu}) = \int d\boldsymbol{p}\left[\mathcal{U}_{\text{ill}}(\boldsymbol{p};\bar{\nu})\sqrt{B_o(\boldsymbol{p};\bar{\nu})}\, h_{vd}(\boldsymbol{x};\boldsymbol{p},\bar{\nu})\right] \tag{13}$$

The definition of the various terms in Eq.(13) is furnished below:

$$\mathcal{U}_{\text{ill}}(\boldsymbol{p};\bar{\nu}) \stackrel{\text{def}}{=} \left(\frac{\bar{\nu}}{ic}\right)\left[\int d\boldsymbol{s}\,\mathcal{A}(\boldsymbol{s};\bar{\nu})\frac{\exp\left(i2\pi\frac{\bar{\nu}}{c}[\|\boldsymbol{s}-\boldsymbol{p}\|]\right)}{\|\boldsymbol{s}-\boldsymbol{p}\|}\psi(\boldsymbol{s},\boldsymbol{p})\right]$$

complex-valued speckle illumination incident on the object point $\boldsymbol{p}$, due to scattering at the Virtual Source.

$$h_{vd}(\boldsymbol{x};\boldsymbol{p},\bar{\nu}) \stackrel{\text{def}}{=} \left(\frac{\bar{\nu}}{ic}\right)\left[\int d\boldsymbol{w}\left(\frac{\exp\left(i2\pi\frac{\bar{\nu}}{c}\|\boldsymbol{p}-\boldsymbol{w}\|\right)}{\|\boldsymbol{p}-\boldsymbol{w}\|}\psi(\boldsymbol{p},\boldsymbol{w})\right)\sqrt{R_{vd}(\boldsymbol{w};\bar{\nu})}\, h_{\text{blur}}(\boldsymbol{x};\boldsymbol{w},\bar{\nu})\right]$$

Speckle point-spread-function (PSF) of light transport from the obscured object point $\boldsymbol{p}$ to a point $\boldsymbol{x}$ on the sensor plane, following a scattering event at the Virtual Detector.

The reformulation helps draw parallels between conventional imaging using physical sources/detectors and indirect imaging using vitualized sources/detectors. The term $\mathcal{U}_{\text{ill}}(\boldsymbol{p};\bar{\nu})$ represents the incident illumination on the obscured object, while $h_{vd}(\boldsymbol{x};\boldsymbol{p},\bar{\nu})$ represents the PSF associated with light transport from the object to the sensor. The PSF $h_{vd}(\boldsymbol{x};\boldsymbol{p},\bar{\nu})$ represents the combined influence of scattering at the Virtual Detector relay wall and blurring intrinsic to optical imaging. As a result, the indirect imaging PSF $h_{vd}(\boldsymbol{x};\boldsymbol{p},\bar{\nu})$ is stochastic in character, and its structure depends on the unknown roughness profile of the Virtual Detector surface.

## 1.4 Expression for sampled hologram recorded by Lock-In sensor

At this point, we have the necessary ingredients to identify the expression for the sampled hologram recorded by the Lock-In sensor. It is obtained by incorporating the expression for the obscured object field $\mathcal{U}_o(\boldsymbol{x};\bar{\nu})$ identified in Eq.(13) into Eq.(11). The resulting expression is shown below:

$$\mathcal{U}_\Delta[\boldsymbol{n};\bar{\nu}] = \frac{N}{\nu_b}\mathcal{U}_r^*[\boldsymbol{n};\bar{\nu}]\left\{\int_{(\boldsymbol{n}-0.5F)\Delta}^{(\boldsymbol{n}+0.5F)\Delta} d\boldsymbol{x}\,\mathcal{U}_o(\boldsymbol{x};\bar{\nu})\right\}$$

$$= \frac{N}{\nu_b}\mathcal{U}_r^*[\boldsymbol{n};\bar{\nu}]\left\{\int_{(\boldsymbol{n}-0.5F)\Delta}^{(\boldsymbol{n}+0.5F)\Delta} d\boldsymbol{x}\left(\int d\boldsymbol{w}\left(\int d\boldsymbol{p}\sqrt{B_o(\boldsymbol{p};\bar{\nu})}\left(\int d\boldsymbol{s}\,\mathcal{A}(\boldsymbol{s};\bar{\nu})\frac{\exp\left(i2\pi\frac{\bar{\nu}}{c}[\|\boldsymbol{s}-\boldsymbol{p}\|+\|\boldsymbol{p}-\boldsymbol{w}\|]\right)}{\|\boldsymbol{s}-\boldsymbol{p}\|\times\|\boldsymbol{p}-\boldsymbol{w}\|}\psi_{sp}\psi_{pw}\right)\right)\sqrt{R_{vd}(\boldsymbol{w};\bar{\nu})}\,h_{\text{blur}}(\boldsymbol{x};\boldsymbol{w},\bar{\nu})\right)\right\} \quad (14)$$

$$= \frac{N}{\nu_b}\mathcal{U}_r^*[\boldsymbol{n};\bar{\nu}]\left\{\int d\boldsymbol{p}\left(\mathcal{U}_{\text{ill}}(\boldsymbol{p};\bar{\nu})\sqrt{B_o(\boldsymbol{p};\bar{\nu})}\right)\left(\int_{(\boldsymbol{n}-0.5F)\Delta}^{(\boldsymbol{n}+0.5F)\Delta} d\boldsymbol{x}\,h_{vd}(\boldsymbol{x};\boldsymbol{p},\bar{\nu})\right)\right\} \quad (15)$$

The innermost nested integrals in Eq. (14) represent the sum of elementary phasors associated with each ray path originating at the Virtual Source, bouncing off the obscured object and terminating at the $\boldsymbol{n}^{th}$ Virtual Detector pixel. The spatial extent of the $\boldsymbol{n}^{th}$ Virtual Detector pixel is determined by the geometric image of the $\boldsymbol{n}^{th}$ physical detector pixel (IFOV).

The integral identity of Eq.(15) recasts the expression for the sampled hologram in a mathematical form that closely resembles the standard space-variant imaging formulation [7]. The term within blue brackets captures the effect of detector aliasing, and describes the number of speckle cells within the PSF $h_{vd}(\boldsymbol{x};\boldsymbol{p},\bar{\nu})$ that can be accommodated in a single detector pixel. This number should not be excessively large ($< 10$) to avoid amplitude/signal fading due to coherent averaging of speckle amplitudes within a pixel [4].

It is also evident from Eq.(15) that the optical hologram recorded by the physical detector does not exhibit any deterministic relationship to the obscured object field $\mathcal{U}_{\text{ill}}(\boldsymbol{p};\bar{\nu})\sqrt{B_o(\boldsymbol{p};\bar{\nu})}$. This is due in large part to the stochastic character of the PSF $h_{vd}(\boldsymbol{x};\boldsymbol{p},\bar{\nu})$, and the additional randomization imposed by integration of the PSF within each sensor pixel. Fortunately, it is possible under restricted conditions, to recover a holographic representation of the obscured object by computational mixing of the sampled hologram at $\bar{\nu}$ with a second hologram acquired at a closely spaced frequency $\bar{\nu}+\Delta\nu$. The remainder of this section identifies the conditions under which a latent hologram of the obscured object may be recovered.

We begin by identifying the expression for the sampled hologram at the second optical frequency $\bar{\nu}+\Delta\nu$, and is disclosed below:

$$\mathcal{U}_\Delta[\boldsymbol{n};\bar{\nu}+\Delta\nu] = \frac{N}{\nu_b}\mathcal{U}_r^*[\boldsymbol{n};\bar{\nu}+\Delta\nu]\left\{\int_{(\boldsymbol{n}-0.5F)\Delta}^{(\boldsymbol{n}+0.5F)\Delta} d\boldsymbol{x}\,\mathcal{U}_o(\boldsymbol{x};\bar{\nu}+\Delta\nu)\right\}$$

$$= \frac{N}{\nu_b}\mathcal{U}_r^*[\boldsymbol{n};\bar{\nu}+\Delta\nu]\left\{\int d\boldsymbol{p}\left(\mathcal{U}_{\text{ill}}(\boldsymbol{p};\bar{\nu}+\Delta\nu)\sqrt{B_o(\boldsymbol{p};\bar{\nu}+\Delta\nu)}\right)\left(\int_{(\boldsymbol{n}-0.5F)\Delta}^{(\boldsymbol{n}+0.5F)\Delta} d\boldsymbol{x}\,h_{vd}(\boldsymbol{x};\boldsymbol{p},\bar{\nu}+\Delta\nu)\right)\right\} \quad (16)$$

The definition of the various terms in Eq.(16) mirrors Eq.(13), and is restated for the benefit of the reader:

$$\mathcal{U}_{\text{ill}}(\boldsymbol{p};\bar{\nu}+\Delta\nu) \stackrel{\text{def}}{=} \left(\frac{\bar{\nu}+\Delta\nu}{ic}\right)\left(\int d\boldsymbol{s}\,\mathcal{A}(\boldsymbol{s};\bar{\nu}+\Delta\nu)\frac{\exp\left(i2\pi\frac{\bar{\nu}+\Delta\nu}{c}[\|\boldsymbol{s}-\boldsymbol{p}\|]\right)}{\|\boldsymbol{s}-\boldsymbol{p}\|}\psi(\boldsymbol{s},\boldsymbol{p})\right)$$

$$h_{vd}(\boldsymbol{x};\boldsymbol{p},\bar{\nu}+\Delta\nu) \stackrel{\text{def}}{=} \left(\frac{\bar{\nu}+\Delta\nu}{ic}\right)\left[\int d\boldsymbol{w}\left(\frac{\exp\left(i2\pi\frac{\bar{\nu}+\Delta\nu}{c}\|\boldsymbol{p}-\boldsymbol{w}\|\right)}{\|\boldsymbol{p}-\boldsymbol{w}\|}\psi(\boldsymbol{p},\boldsymbol{w})\right)\sqrt{R_{vd}(\boldsymbol{w};\bar{\nu}+\Delta\nu)}\, h_{\text{blur}}(\boldsymbol{x};\boldsymbol{w},\bar{\nu}+\Delta\nu)\right]$$

Examination of the expressions for the sampled holograms disclosed in Eqs.(15),(16) fails to divulge any obvious relation between the detected fields at the two closely spaced optical frequencies $\bar{\nu}$ and $\bar{\nu}+\Delta\nu$. The relation between the sampled holograms may be elucidated by making simplifying assumptions regarding the indirect imaging geometry and the scattering properties of the Virtual Source/Detector surfaces. These assumptions are enumerated below:

A1. $\mathcal{A}(\boldsymbol{s};\bar{\nu}+\Delta\nu) = \mathcal{A}(\boldsymbol{s};\bar{\nu})$ — *Spectral reflectance of Virtual Source surface is unchanged for small change in optical frequency*

A2. $B_o(\boldsymbol{p};\bar{\nu}+\Delta\nu) = B_o(\boldsymbol{p};\bar{\nu})$ — *Object albedo is unchanged for small change in optical frequency*

A3. $R_{vd}(\boldsymbol{p};\bar{\nu}+\Delta\nu) = R_{vd}(\boldsymbol{p};\bar{\nu})$ — *Virtual Detector albedo is unchanged for small change in optical frequency*

A4. $\mathcal{U}_r[\boldsymbol{n};\bar{\nu}+\Delta\nu] = \mathcal{U}_r[\boldsymbol{n};\bar{\nu}]$ — *Phase fluctuations induced by a small change in the optical frequency of the reference beam are negligibly small*

A5. *The Virtual Source subtends a small solid angle with respect to the object,* so that a small change in the optical frequency of the CW source induces a proportional change in the optical path length (OPL) of ray paths $\overrightarrow{\boldsymbol{sp}}$ originating at a point $\boldsymbol{s}$ on the Virtual Source and terminating at the object point $\boldsymbol{p}$. The excess phase induced by the change in OPL is given below:

$$\Phi(\overrightarrow{\boldsymbol{sp}};\Delta\nu) \stackrel{\text{def}}{=} 2\pi\left(\left(\frac{\bar{\nu}+\Delta\nu}{c}\right)\|\boldsymbol{s}-\boldsymbol{p}\|\right)-\left(\left(\frac{\bar{\nu}}{c}\right)\|\boldsymbol{s}-\boldsymbol{p}\|\right) = 2\pi\left(\frac{\Delta\nu}{c}\right)\|\boldsymbol{s}-\boldsymbol{p}\|$$

$$\approx 2\pi\left(\frac{\Delta\nu}{c}\right)\|\bar{\boldsymbol{s}}-\boldsymbol{p}\|\left(1+\frac{1}{2}\frac{\|\boldsymbol{s}-\bar{\boldsymbol{s}}\|^2}{\|\bar{\boldsymbol{s}}-\boldsymbol{p}\|^2}+\frac{(\boldsymbol{s}-\bar{\boldsymbol{s}})^T(\bar{\boldsymbol{s}}-\boldsymbol{p})}{\|\bar{\boldsymbol{s}}-\boldsymbol{p}\|^2}\right) \quad (17)$$

$$\approx 2\pi\left(\frac{\Delta\nu}{c}\right)\|\bar{\boldsymbol{s}}-\boldsymbol{p}\|+\epsilon \quad (18)$$

where $\bar{\boldsymbol{s}}$ is a fixed point on the Virtual Source surface, such as the centroid of the VS. The assumption of small solid-angle is evidenced in the binomial approximation of Eq.(17).

The first term in Eq.(18) is the phase associated with a spherical wave at the notional wavelength (or synthetic wavelength) $c\Delta\nu^{-1}$ meters. It encodes the position of the obscured object from the vantage point of the Virtual Source. The second term $\epsilon$ in Eq.(18) is the excess phase or wavefront aberration induced by a change in the optical frequency. The term is dominated by the phase component $2\pi\left(\frac{\Delta\nu}{c}\right)(\boldsymbol{s}-\bar{\boldsymbol{s}})^T\left(\frac{\bar{\boldsymbol{s}}-\boldsymbol{p}}{\|\bar{\boldsymbol{s}}-\boldsymbol{p}\|}\right)$. The wavefront error imparted by this component is negligible so long as $|\epsilon| \ll 1$ radian [3], for each ray-path $\overrightarrow{\boldsymbol{sp}}$ originating at the Virtual Source and terminating at the obscured object point $\boldsymbol{p}$. As a result,

$$|\epsilon| \ll 1 \quad \Rightarrow \quad \left(\frac{\Delta\nu}{c}\right)\left|(\boldsymbol{s}-\bar{\boldsymbol{s}})^T\left(\frac{\bar{\boldsymbol{s}}-\boldsymbol{p}}{\|\bar{\boldsymbol{s}}-\boldsymbol{p}\|}\right)\right| \ll \frac{1}{2\pi} \quad (19)$$

$$\therefore \quad \|\boldsymbol{s}-\bar{\boldsymbol{s}}\|\left|\left(\frac{\boldsymbol{s}-\bar{\boldsymbol{s}}}{\|\boldsymbol{s}-\bar{\boldsymbol{s}}\|}\right)^T\left(\frac{\bar{\boldsymbol{s}}-\boldsymbol{p}}{\|\bar{\boldsymbol{s}}-\boldsymbol{p}\|}\right)\right| \ll \frac{c\Delta\nu^{-1}}{2\pi} \quad \Rightarrow \quad \|\boldsymbol{s}-\bar{\boldsymbol{s}}\| < \frac{c\Delta\nu^{-1}}{2\pi}$$

$$\|\boldsymbol{s}-\bar{\boldsymbol{s}}\| \approx \sqrt{\left(\frac{\emptyset_{vs}}{2}\right)^2+{\sigma_h}^2} \quad \text{so that} \quad \sqrt{\left(\frac{\emptyset_{vs}}{2}\right)^2+\sigma_h^2} < \frac{c\Delta\nu^{-1}}{8} < \frac{c\Delta\nu^{-1}}{2\pi} \quad (20)$$

where-in $\emptyset_{vs}$ reperesents the diameter of the illumination beam incident on the Virtual Source surface and $\sigma_h$ represents the RMS roughness of the Virtual Source surface. The term $c\Delta\nu^{-1}$

represents the change in wavelength resulting from a change in the optical frequency of the CW source by $\Delta\nu$ Hz. In deriving Eq.(20), the wavenumber associated with the synthetic wavelength $2\pi(c^{-1}\Delta\nu)$ is approximated as $8(c^{-1}\Delta\nu)$ meter$^{-1}$.

The empirical bound of Eq.(20) divulges a tradeoff between the maximum permitted frequency shift $\Delta\nu$, and the choice of beam waist and RMS roughness of the Virtual Source surface. For a Virtual Source surface with approximate knowledge of the RMS roughness, a larger frequency shift may only be admitted by reducing the size of the Virtual Source, a fact borne out in experiments.

A6. *A small change $\Delta\nu$ in the optical frequency of the CW illumination source induces longitudinal chromatic aberration in the diffraction limited optical blur at $\bar{\nu}$*, and is expressed as follows:

$$h_{\text{blur}}\left(\boldsymbol{x} \stackrel{\text{def}}{=} \begin{bmatrix} x_1 \\ x_2 \end{bmatrix}; \boldsymbol{w} \stackrel{\text{def}}{=} \begin{bmatrix} w_1 \\ w_2 \\ w_3 \end{bmatrix}, \bar{\nu} + \Delta\nu\right) \approx \left(\frac{\bar{\nu} + \Delta\nu}{\bar{\nu}}\right)^2 \left[\exp\left(i\frac{2\pi\Delta\nu}{c}\left[z_d + \frac{[x_1^2 + x_2^2]}{2z_d} + \bar{w}_3 + \frac{[w_1^2 + w_2^2]}{2\bar{w}_3}\right]\right)\right] h_{\text{blur}}(\boldsymbol{x}; \boldsymbol{w}, \bar{\nu}) \tag{21}$$

The term $\bar{w}_3$ represents the mean distance from the VD surface to the entrance pupil plane of the imaging optic. The approximation is valid so long as the peak-valley height fluctuations in the Virtual Detector surface are smaller than $\frac{1}{8^{\text{th}}}$ change in the wavelength of the interrogation source, namely $c\Delta\nu^{-1}$ meters. A formal proof is furnished in Section-0.

- *Finite extent of each detector pixel:* Over the finite extent of the $\boldsymbol{n}^{th}$ detector pixel, the quadratic phase variation $\frac{2\pi\Delta\nu}{c}\frac{\|\boldsymbol{x}\|^2}{2z_d}$ imparted by the longitudinal chromatic aberration in the optical blur of Eq.(21), can be approximated by the complex valued constant shown below:

$$\frac{2\pi\Delta\nu}{c}\frac{\|\boldsymbol{x}\|^2}{2z_d} \approx \frac{2\pi\Delta\nu}{c}\frac{\|\boldsymbol{n\Delta}\|^2}{2z_d} \qquad \forall \boldsymbol{x} \in (\boldsymbol{n}\Delta - \boldsymbol{0.5}F\Delta, \boldsymbol{n}\Delta + \boldsymbol{0.5}F\Delta) \tag{22}$$

- *Finite extent of the optical blur:* The finite spatial extent of the optical blur $h_{\text{blur}}$ limits the set of Virtual Detector locations $\boldsymbol{w}$: $(w_1, w_2, w_3)$ that contribute to the integrated field amplitude at the $\boldsymbol{n}^{th}$ detector pixel. These locations are confined to a small region in the vicinity of the geometric image of the center of the $\boldsymbol{n}^{th}$ detector pixel, as observed on the Vitual Detector surface. Thus, the position vector $[w_1, w_2, w_3]^T$ associated with a point on the VD surface may instead be approximated by the vector $[-z_d^{-1}\bar{w}_3\boldsymbol{n}\Delta \quad \bar{w}_3]^T$, for all $\boldsymbol{x} \in (\boldsymbol{n}\Delta - \boldsymbol{0.5}F\Delta, \boldsymbol{n}\Delta + \boldsymbol{0.5}F\Delta)$. The scalar $z_d^{-1}\bar{w}_3$ in the approximation represents the transverse magnification associated with the imaging identity of Eq.(1), and $\bar{w}_3$ is the mean perpendicular distance from the VD surface to the entrance pupil plane of the imaging optics. As a consequence of this approximation, the quadratic phase variations $\frac{2\pi\Delta\nu}{c}\frac{[w_1^2+w_2^2]}{2\bar{w}_3}$ imparted by the longitudinal chromatic aberration in the optical blur of Eq.(21), can be approximated by the complex valued constant shown below

$$\frac{2\pi\Delta\nu}{c}\frac{[w_1^2 + w_2^2]}{2\bar{w}_3} \approx \frac{2\pi\Delta\nu}{c}\frac{\|z_d^{-1}\bar{w}_3\boldsymbol{n}\Delta\|^2}{2\bar{w}_3} \qquad \forall \boldsymbol{x} \in (\boldsymbol{n}\Delta - \boldsymbol{0.5}F\Delta, \boldsymbol{n}\Delta + \boldsymbol{0.5}F\Delta) \tag{23}$$

A7. *Each Virtual Detector pixel subtends a small solid angle with respect to the object,* so that change a small change in the optical frequency of the CW source induces a proportional change in the optical path length (OPL) of ray paths $\overrightarrow{\boldsymbol{pw}}$ originating at a point $\boldsymbol{p}$ on the obscured object and terminating at the point $\boldsymbol{w}$ on the Virtual Detector surface. The excess phase induced by the change in OPL is given below:

$$\Phi(\overrightarrow{\boldsymbol{pw}};\Delta\nu) \stackrel{\text{def}}{=} 2\pi\left(\left(\frac{\bar{\nu}+\Delta\nu}{c}\right)\|\boldsymbol{p}-\boldsymbol{w}\|\right)-\left(\left(\frac{\bar{\nu}}{c}\right)\|\boldsymbol{p}-\boldsymbol{w}\|\right)=2\pi\left(\frac{\Delta\nu}{c}\right)\|\boldsymbol{p}-\boldsymbol{w}\|$$

$$\approx 2\pi\left(\frac{\Delta\nu}{c}\right)\left\|\boldsymbol{p}-\begin{bmatrix}-z_d^{-1}\bar{w}_3\boldsymbol{n}\Delta\\ \bar{w}_3\end{bmatrix}\right\|\left(1+\frac{1}{2}\frac{\left\|\begin{bmatrix}-z_d^{-1}\bar{w}_3\boldsymbol{n}\Delta\\ \bar{w}_3\end{bmatrix}-\boldsymbol{w}\right\|^2}{\left\|\boldsymbol{p}-\begin{bmatrix}-z_d^{-1}\bar{w}_3\boldsymbol{n}\Delta\\ \bar{w}_3\end{bmatrix}\right\|^2}+\frac{\left(\begin{bmatrix}-z_d^{-1}\bar{w}_3\boldsymbol{n}\Delta\\ \bar{w}_3\end{bmatrix}-\boldsymbol{w}\right)^T\left(\boldsymbol{p}-\begin{bmatrix}-z_d^{-1}\bar{w}_3\boldsymbol{n}\Delta\\ \bar{w}_3\end{bmatrix}\right)}{\left\|\boldsymbol{p}-\begin{bmatrix}-z_d^{-1}\bar{w}_3\boldsymbol{n}\Delta\\ \bar{w}_3\end{bmatrix}\right\|^2}\right) \quad (24)$$

$$\approx 2\pi\left(\frac{\Delta\nu}{c}\right)\left\|\boldsymbol{p}-\begin{bmatrix}-z_d^{-1}\bar{w}_3\boldsymbol{n}\Delta\\ \bar{w}_3\end{bmatrix}\right\|+\epsilon \quad (25)$$

where $\begin{bmatrix}-z_d^{-1}\bar{w}_3\boldsymbol{n}\Delta\\ \bar{w}_3\end{bmatrix}$ is the geometric center of the $\boldsymbol{n}^{th}$ Virtual Detector pixel. The assumption of small solid-angle is evidenced in the binomial approximation of Eq.(24).

The first term in Eq.(25) is the phase associated with a spherical wave at the notional wavelength (or synthetic wavelength) $c\Delta\nu^{-1}$ meters. It encodes the position of the obscured object from the vantage point of the Virtual Detector, and is essential to recovering a holographic description of the obscured object. The second term $\epsilon$ in Eq. (25) is the excess phase or wavefront aberration induced by a change in the optical frequency. The term is dominated by the third component within blue brackets. The wavefront error imparted by this component is negligible so long as $|\epsilon| \ll 1$ radian [3], for each ray-path $\overrightarrow{\boldsymbol{pw}}$ originating at the obscured object point $\boldsymbol{p}$ and terminating in the $\boldsymbol{n}^{th}$Virtual Detector pixel. As a result,

$$|\epsilon| \ll 1 \quad \Rightarrow \quad \left(\frac{\Delta\nu}{c}\right)\left(\left(\begin{bmatrix}-z_d^{-1}\bar{w}_3\boldsymbol{n}\Delta\\ \bar{w}_3\end{bmatrix}-\boldsymbol{w}\right)^T\left(\frac{\boldsymbol{p}-\begin{bmatrix}-z_d^{-1}\bar{w}_3\boldsymbol{n}\Delta\\ \bar{w}_3\end{bmatrix}}{\left\|\boldsymbol{p}-\begin{bmatrix}-z_d^{-1}\bar{w}_3\boldsymbol{n}\Delta\\ \bar{w}_3\end{bmatrix}\right\|}\right)\right) \ll \frac{1}{2\pi} \quad (26)$$

$$\therefore \quad \left\|\begin{bmatrix}-z_d^{-1}\bar{w}_3\boldsymbol{n}\Delta\\ \bar{w}_3\end{bmatrix}-\boldsymbol{w}\right\|\left(\left(\frac{\begin{bmatrix}-z_d^{-1}\bar{w}_3\boldsymbol{n}\Delta\\ \bar{w}_3\end{bmatrix}-\boldsymbol{w}}{\left\|\begin{bmatrix}-z_d^{-1}\bar{w}_3\boldsymbol{n}\Delta\\ \bar{w}_3\end{bmatrix}-\boldsymbol{w}\right\|}\right)^T\left(\frac{\boldsymbol{p}-\begin{bmatrix}-z_d^{-1}\bar{w}_3\boldsymbol{n}\Delta\\ \bar{w}_3\end{bmatrix}}{\left\|\boldsymbol{p}-\begin{bmatrix}-z_d^{-1}\bar{w}_3\boldsymbol{n}\Delta\\ \bar{w}_3\end{bmatrix}\right\|}\right)\right) \ll \frac{c\Delta\nu^{-1}}{2\pi}$$

$$\Rightarrow \quad \left\|\begin{bmatrix}-z_d^{-1}\bar{w}_3\boldsymbol{n}\Delta\\ \bar{w}_3\end{bmatrix}-\boldsymbol{w}\right\| < \frac{c\Delta\nu^{-1}}{2\pi}$$

$$\left\|\begin{bmatrix}-z_d^{-1}\bar{w}_3\boldsymbol{n}\Delta\\ \bar{w}_3\end{bmatrix}-\boldsymbol{w}\right\| \approx \sqrt{\left(\frac{z_d^{-1}\bar{w}_3F\Delta}{2}\right)^2+\sigma_h^2} \quad \text{so that} \quad \sqrt{\left(\frac{z_d^{-1}\bar{w}_3F\Delta}{2}\right)^2+\sigma_h^2} < \frac{c\Delta\nu^{-1}}{8} \quad (27)$$

where-in $z_d^{-1}\bar{w}_3F\Delta$ represents the axtive area of the $\boldsymbol{n}^{th}$ Virtual Detector pixel and and $\sigma_h$ represents the RMS roughness of the Virtual Detector surface. The term $c\Delta\nu^{-1}$ represents the change in wavelength resulting from a change in the optical frequency of the CW source by $\Delta\nu$ Hz. In deriving Eq.(27), the wavenumber associated with the synthetic wavelength $2\pi(c^{-1}\Delta\nu)$ is approximated as $8(c^{-1}\Delta\nu)$ meter$^{-1}$.

The empirical bound of Eq.(27) divulges a tradeoff between the maximum permitted frequency shift $\Delta\nu$, and the size of a Virtual Detector pixel and RMS roughness of the Virtual Source surface. For a Virtual Detector surface with approximate knowledge of the RMS roughness, a larger frequency shift may only be admitted by reducing the size of a Virtual Detector pixel, a fact borne out in experiments.

The primary consequences of the simplifying assumptions of A1-A7 are enumerated below,

- *Field propagation from Virtual Source to obscured object:* A small change $\Delta\nu$ in the optical frequency of the CW source induces a proportional change in the OPL of ray paths $\overrightarrow{\boldsymbol{sp}}$ originating at a point $\boldsymbol{s}$

on the VS and terminating at the object point $\boldsymbol{p}$. The change in OPL can be approximated as $\|\bar{\boldsymbol{s}} - \boldsymbol{p}\|$, where $\bar{\boldsymbol{s}}$ is a fixed point such as the centroid of the illuminated region that makes up the Virtual Source.

- *Field propagation from obscured object to Virtual Detector:* A small change $\Delta\nu$ in the optical frequency of the CW source induces a proportional change in the OPL of ray paths $\overrightarrow{\boldsymbol{pw}}$ originating at a point $\boldsymbol{p}$ on the obscured object and terminating at the point $\boldsymbol{w}$ on the Virtual Detector surface. The change can be approximated as $\left\|\boldsymbol{p} - \begin{bmatrix} -z_d^{-1}\bar{w}_3\boldsymbol{n}\Delta \\ \bar{w}_3 \end{bmatrix}\right\|$, where $\begin{bmatrix} -z_d^{-1}\bar{w}_3\boldsymbol{n}\Delta \\ \bar{w}_3 \end{bmatrix}$ is the geometric center of the $n^{th}$ Virtual Detector pixel (geometric image of center of the $n^{th}$ detector pixel on the Virtual Detector surface).
- *Field propagation from Virtual Detector to image sensor:* A small change $\Delta\nu$ in the optical frequency of the CW source induces longitudinal chromatic aberration in the diffraction limited optical blur associated with imaging the Virtual Detector surface at $\bar{\nu}$. The phase fluctuations due to chromatic aberration may be approximated as $\frac{2\pi\Delta\nu}{c}\left(\frac{\|z_d^{-1}\bar{w}_3\boldsymbol{n}\Delta\|^2}{2\bar{w}_3} + \frac{\|\boldsymbol{n}\Delta\|^2}{2z_d}\right)$ where-in
  - $z_d^{-1}\bar{w}_3$ is the transverse magnification of the imager,
  - $\bar{w}_3$ is the mean perpendicular distance from the VD surface to the entrance pupil plane of the imaging optics,
  - $z_d$ is the distance from the sensor plane to the exit pupil plane of the imaging optics.

### *1.5 Redundant information in the digital holograms at optical frequencies $\bar{\nu}$ and $\bar{\nu} + \Delta\nu$*

A crucial step in assembling the holographic description of the obscured objects is identifying redundant information in the complex-valued holograms recorded at the optical frequencies $\bar{\nu}$ and $\bar{\nu} + \Delta\nu$. To this end, we impose the restrictions A1-A7 upon the expressions for the indirect illumination $\mathcal{U}_{\text{ill}}$ and the indirect imager PSF $h_{vd}$ . The expressions relating the indirect illumination at the two optical frequencies is disclosed below:

$$\mathcal{U}_{\text{ill}}(\boldsymbol{p}; \bar{\nu} + \Delta\nu) \stackrel{\text{def}}{=} \left(\frac{\bar{\nu} + \Delta\nu}{ic}\right) \int d\boldsymbol{s}\, \mathcal{A}(\boldsymbol{s}; \bar{\nu} + \Delta\nu) \frac{\exp\left(i2\pi \frac{\bar{\nu} + \Delta\nu}{c}[\|\boldsymbol{s} - \boldsymbol{p}\|]\right)}{\|\boldsymbol{s} - \boldsymbol{p}\|} \psi(\boldsymbol{s}, \boldsymbol{p})$$

$$= \left(\frac{\bar{\nu} + \Delta\nu}{\bar{\nu}}\right) \times \exp\left(i\frac{2\pi\Delta\nu}{c}\|\bar{\boldsymbol{s}} - \boldsymbol{p}\|\right)\left\{\left(\frac{\bar{\nu}}{ic}\right) \int d\boldsymbol{s}\, \mathcal{A}(\boldsymbol{s}; \bar{\nu}) \frac{\exp\left(i2\pi \frac{\bar{\nu}}{c}[\|\boldsymbol{s} - \boldsymbol{p}\|]\right)}{\|\boldsymbol{s} - \boldsymbol{p}\|} \psi(\boldsymbol{s}, \boldsymbol{p})\right\}$$

$$= \left(\frac{\bar{\nu} + \Delta\nu}{\bar{\nu}}\right) \times \exp\left(i\frac{2\pi\Delta\nu}{c}\|\bar{\boldsymbol{s}} - \boldsymbol{p}\|\right) \times \mathcal{U}_{\text{ill}}(\boldsymbol{p}; \bar{\nu}) \qquad (28)$$

It is evident from Eq.(28) that a small change in optical frequency of the CW source imparts a spherical phase to the field incident on the obscured object point $\boldsymbol{p}$. The excess phase depends on the propagation distance from the centroid of the Virtual Source to the obscured object point, and the incremental change in the wavelength of the CW source (given by $c\Delta\nu^{-1}$ meters). The phase encodes the position of the obscured object from the vantage point of the Virtual Source. (***Observation-1***)

In a similar fashion, it can be shown (Eq.(29)) that a small change in the optical frequency imparts additional spherical phase to the indirect imager PSF associated with each obscured object point $\boldsymbol{p}$.

$$h_{vd}(\boldsymbol{x};\boldsymbol{p},\bar{\nu}+\Delta\nu) \stackrel{\text{def}}{=} \left(\frac{\bar{\nu}+\Delta\nu}{ic}\right)\int d\boldsymbol{w}\left(\frac{\exp\left(i2\pi\frac{\bar{\nu}+\Delta\nu}{c}\|\boldsymbol{p}-\boldsymbol{w}\|\right)}{\|\boldsymbol{p}-\boldsymbol{w}\|}\psi(\boldsymbol{p},\boldsymbol{w})\right)\sqrt{R_{vd}(\boldsymbol{w};\bar{\nu}+\Delta\nu)}\,h_{\text{blur}}(\boldsymbol{x};\boldsymbol{w},\bar{\nu}+\Delta\nu)$$

$$= \left(\frac{\bar{\nu}+\Delta\nu}{\bar{\nu}}\right)^3 \times \left\{\exp\left(i\frac{2\pi\Delta\nu}{c}\left[\left\|\boldsymbol{p}-\begin{bmatrix}-z_d^{-1}\bar{w}_3\boldsymbol{n}\Delta\\ \bar{w}_3\end{bmatrix}\right\| + z_d + \frac{\|\boldsymbol{n}\Delta\|^2}{2z_d} + \bar{w}_3 + \frac{\|z_d^{-1}\bar{w}_3\boldsymbol{n}\Delta\|^2}{2\bar{w}_3}\right]\right)\right\}$$

$$\times\left\{\int d\boldsymbol{w}\left(\frac{\exp\left(i2\pi\frac{\bar{\nu}}{c}\|\boldsymbol{p}-\boldsymbol{w}\|\right)}{\|\boldsymbol{p}-\boldsymbol{w}\|}\psi(\boldsymbol{p},\boldsymbol{w})\right)\sqrt{R_{vd}(\boldsymbol{w};\bar{\nu})}\,h_{\text{blur}}(\boldsymbol{x};\boldsymbol{w},\bar{\nu})\right\}$$

$$= \left(\frac{\bar{\nu}+\Delta\nu}{\bar{\nu}}\right)^3 \times \left\{\exp\left(i\frac{2\pi\Delta\nu}{c}\left(\left\|\boldsymbol{p}-\begin{bmatrix}-z_d^{-1}\bar{w}_3\boldsymbol{n}\Delta\\ \bar{w}_3\end{bmatrix}\right\| + z_d + \frac{\|\boldsymbol{n}\Delta\|^2}{2z_d} + \bar{w}_3 + \frac{\|z_d^{-1}\bar{w}_3\boldsymbol{n}\Delta\|^2}{2\bar{w}_3}\right)\right)\right\} h_{vd}(\boldsymbol{x};\boldsymbol{p},\bar{\nu}) \quad (29)$$

The additional phase contribution highlighted in yellow varies with the propagation distance from the obscured object point $\boldsymbol{p}$ to the center of the $\boldsymbol{n}^{th}$ Virtual Detector pixel. The excess phase contribution highligted in blue varies with the length of the chief ray originating at the center of the $\boldsymbol{n}^{th}$ Virtual Detector pixel and terminating at the center of $\boldsymbol{n}^{th}$ sensor pixel.

A small change in the optical frequency of the CW source imparts a spherical phase to the impulse response of the indirect imager. The excess phase depends on the incremental change in the wavelength of the CW source (given by $c\Delta\nu^{-1}$ meters), and the cumulative propagation distance from the obscured object point to the center of the $\boldsymbol{n}^{th}$ Virtual Detector and sensor pixels. (***Observation-2)***

Incorporating Eqs.(28)-(29) into Eq.(16) yields the following revised expression for the sampled hologram at the optical frequency $\bar{\nu}+\Delta\nu$:

$$\mathcal{U}_\Delta[\boldsymbol{n};\bar{\nu}+\Delta\nu]$$

$$= \left(\frac{\bar{\nu}+\Delta\nu}{\bar{\nu}}\right)^4 \frac{N}{\nu_b}\mathcal{U}_r^*[\boldsymbol{n};\bar{\nu}]\exp(i\phi[\boldsymbol{n};\Delta\nu])\left\{\int d\boldsymbol{p}\left(\exp(i\theta[\boldsymbol{n};\boldsymbol{p},\Delta\nu])\left(\mathcal{U}_{\text{ill}}(\boldsymbol{p};\bar{\nu})\sqrt{B_o(\boldsymbol{p};\bar{\nu})}\left(\int_{(\boldsymbol{n}-0.5F)\Delta}^{(\boldsymbol{n}+0.5F)\Delta} d\boldsymbol{x}\, h_{vd}(\boldsymbol{x};\boldsymbol{p},\bar{\nu})\right)\right)\right)\right\} \quad (30)$$

The definition of the phasors $\phi[\boldsymbol{n};\Delta\nu]$ and $\theta[\boldsymbol{n};\boldsymbol{p},\Delta\nu]$ is furnished below:

$$\phi[\boldsymbol{n};\Delta\nu] \stackrel{\text{def}}{=} 2\pi\frac{\Delta\nu}{c}\left(z_d + \frac{\|\boldsymbol{n}\Delta\|^2}{2z_d} + \bar{w}_3 + \frac{\|z_d^{-1}\bar{w}_3\boldsymbol{n}\Delta\|^2}{2\bar{w}_3}\right)$$

scene-independent phasor field representing the change in OPL associated with light transport from $\boldsymbol{n}^{\text{th}}$ Virtual Detector pixel to the $\boldsymbol{n}^{th}$ sensor pixel.

$$\theta[\boldsymbol{n};\boldsymbol{p},\Delta\nu] \stackrel{\text{def}}{=} 2\pi\frac{\Delta\nu}{c}\left(\|\bar{\boldsymbol{s}}-\boldsymbol{p}\| + \left\|\boldsymbol{p}-\begin{bmatrix}-z_d^{-1}\bar{w}_3\boldsymbol{n}\Delta\\ \bar{w}_3\end{bmatrix}\right\|\right)$$

scene dependent phasor field representing the change in the OPL of all ray paths originating at the Virtual Source, bouncing off the obscured object and terminating at the $\boldsymbol{n}^{th}$ Virtual Detector pixel.

A small change $\Delta\nu$ in the optical frequency of the CW source used to interrogate the hidden scene imparts an additional spherical phase to the field contribution of each obscured object point $\boldsymbol{p}$. The excess spherical phase encodes the position of the obscured object point $\boldsymbol{p}$ at the "synthetic" wavelength $c\Delta\nu^{-1}$ meters. (***Observation-3***)

### 1.6 Recovering the latent hologram at the synthetic wavelength $c\Delta\nu^{-1}$

Observation-3 forms the basis of our claim (Claim-1) that a holographic description of the obscured object can be recovered despite scattering at the Virtual Source and Virtual Detector surfaces. As a first step

towards corroborating this claim, we seek to computationally mix the sampled holograms at $\bar{\nu}, \bar{\nu}+\Delta\nu$. The resulting expression is shown below:

$$\mathcal{U}_\Delta[\boldsymbol{n},\bar{\nu}] \times \mathcal{U}_\Delta^*[\boldsymbol{n},\bar{\nu}+\Delta\nu]$$
$$= \left(\left(\frac{N}{\nu_b}\right)^2 \mathcal{U}_r[\boldsymbol{n};\bar{\nu}]\,\mathcal{U}_r^*[\boldsymbol{n};\bar{\nu}+\Delta\nu]\right) \times \left\{\left(\int_{(\boldsymbol{n}-0.5F)\Delta}^{(\boldsymbol{n}+0.5F)\Delta} d\boldsymbol{x}\,\mathcal{U}_o(\boldsymbol{x};\bar{\nu})\right) \times \left(\int_{(\boldsymbol{n}-0.5F)\Delta}^{(\boldsymbol{n}+0.5F)\Delta} d\acute{\boldsymbol{x}}\,\mathcal{U}_o^*(\acute{\boldsymbol{x}};\bar{\nu}+\Delta\nu)\right)\right\}$$
$$= \left(\left(\frac{\bar{\nu}+\Delta\nu}{\bar{\nu}}\right)^4 \left(\frac{N}{\nu_b}\right)^2 I_r[\boldsymbol{n};\bar{\nu}]\right) \exp(i\phi[\boldsymbol{n};\Delta\nu]) \left\{\iint d\boldsymbol{p}\,d\acute{\boldsymbol{p}} \left(\begin{matrix}\mathcal{U}_{\text{ill}}(\boldsymbol{p};\bar{\nu})\mathcal{U}_{\text{ill}}^*(\acute{\boldsymbol{p}};\bar{\nu}) \\ \times \sqrt{B_o(\boldsymbol{p};\bar{\nu})B_o(\acute{\boldsymbol{p}};\bar{\nu})}\end{matrix}\right) \exp(i\theta[\boldsymbol{n};\acute{\boldsymbol{p}},\Delta\nu]) \left(\iint_{(\boldsymbol{n}-0.5F)\Delta}^{(\boldsymbol{n}+0.5F)\Delta} d\boldsymbol{x}\,d\acute{\boldsymbol{x}} \left(\begin{matrix}h_{vd}(\boldsymbol{x};\boldsymbol{p},\bar{\nu}) \\ \times h_{vd}^*(\acute{\boldsymbol{x}};\acute{\boldsymbol{p}},\bar{\nu})\end{matrix}\right)\right)\right\} \quad (31)$$

Interchanging the order of integration in Eq.

(31) yields the following expression for the computational hologram:

$$\mathcal{U}_\Delta[\boldsymbol{n},\bar{\nu}] \times \mathcal{U}_\Delta^*[\boldsymbol{n},\bar{\nu}+\Delta\nu]$$
$$= \left(\left(\frac{\bar{\nu}+\Delta\nu}{\bar{\nu}}\right)^4 \left(\frac{N}{\nu_b}\right)^2 I_r[\boldsymbol{n};\bar{\nu}]\right) \left(\begin{matrix} \exp(i\phi[\boldsymbol{n};\Delta\nu]) \int d\boldsymbol{p} \left(|\mathcal{U}_{\text{ill}}(\boldsymbol{p};\bar{\nu})|^2 B_o(\boldsymbol{p};\bar{\nu}) \left|\int_{(\boldsymbol{n}-0.5F)\Delta}^{(\boldsymbol{n}+0.5F)\Delta} d\boldsymbol{x}\,h_{vd}(\boldsymbol{x};\boldsymbol{p},\bar{\nu})\right|^2\right) \exp(i\theta[\boldsymbol{n};p,\Delta\nu]) \; + \quad (32) \\ \exp(i\phi[\boldsymbol{n};\Delta\nu]) \iint_{\boldsymbol{p}\neq\acute{\boldsymbol{p}}} d\boldsymbol{p}\,d\acute{\boldsymbol{p}} \left(\begin{matrix}\mathcal{U}_{\text{ill}}(\boldsymbol{p};\bar{\nu})\mathcal{U}_{\text{ill}}^*(\acute{\boldsymbol{p}};\bar{\nu}) \\ \times \sqrt{B_o(\boldsymbol{p};\bar{\nu})B_o(\acute{\boldsymbol{p}};\bar{\nu})}\end{matrix}\right) \exp(i\theta[\boldsymbol{n};\acute{\boldsymbol{p}},\Delta\nu]) \iint_{(\boldsymbol{n}-0.5F)\Delta}^{(\boldsymbol{n}+0.5F)\Delta} d\boldsymbol{x}\,d\acute{\boldsymbol{x}} \left(\begin{matrix}h_{vd}(\boldsymbol{x};\boldsymbol{p},\bar{\nu}) \\ \times h_{vd}^*(\acute{\boldsymbol{x}};\acute{\boldsymbol{p}},\bar{\nu})\end{matrix}\right) \quad (33)\end{matrix}\right)$$
$$= \mathcal{U}_{\text{latent}}[\boldsymbol{n},\Delta\nu] + \mathcal{U}_{\text{parasitic}}[\boldsymbol{n},\bar{\nu}]$$

Notice that the expression for the computational hologram is comprised of two terms. The first of these terms higlighted in yellow encapsulates spectral intreference of field contributions for a single obscured object point $\boldsymbol{p}$. This term is dubbed the latent hologram as it encodes a holographic description of the obscured object, at the synthetic wavelngth of $\Lambda = c\Delta\nu^{-1}$ meters.

The second term highlighted in gray encapsulates the spectral interference of field contributions of two spatially distinct object points $\boldsymbol{p}, \acute{\boldsymbol{p}}$. This term is a parasitic interference term that complicates the recovery of the latent hologram.

The exact expression for the latent hologram may be identified by incorporating the definition of the scene-dependent and scene-independent phasor fields into the expression for the latent hologram disclosed in Eq(32). The resulting expression is furnished in Eq.(34).

$$\mathcal{U}_{\text{latent}}[\boldsymbol{n};\Delta\nu]$$
$$= \left(\left(\frac{\bar{\nu}+\Delta\nu}{\bar{\nu}}\right)^4 \left(\frac{N}{\nu_b}\right)^2 I_r[\boldsymbol{n};\bar{\nu}]\right) \exp(i\phi[\boldsymbol{n};\Delta\nu]) \int d\boldsymbol{p} \left\{\begin{matrix}\left(|\mathcal{U}_{\text{ill}}(\boldsymbol{p};\bar{\nu})|^2 B_o(\boldsymbol{p};\bar{\nu}) \left|\int_{(\boldsymbol{n}-0.5F)\Delta}^{(\boldsymbol{n}+0.5F)\Delta} d\boldsymbol{x}\,h_{vd}(\boldsymbol{x};\boldsymbol{p},\bar{\nu})\right|^2\right) \\ \exp\left(i2\pi\frac{\Delta\nu}{c}\left(\|\bar{\boldsymbol{s}}-\boldsymbol{p}\| + \left\|\boldsymbol{p} - \begin{bmatrix}-z_d^{-1}\bar{w}_3\boldsymbol{n}\Delta \\ \bar{w}_3\end{bmatrix}\right\|\right)\right)\end{matrix}\right\} \quad (34)$$

The spherical phase factors embedded in Eq.(34) fully encode the position of the obscured object point $\boldsymbol{p}$ at the synthetic wavelength $c\Delta\nu^{-1}$ meters. Consequently, numerical backpropagation of the latent hologram should permit reconstruction of the light distribution in the hiddden volume. However, the ability to localize the obscured object point $\boldsymbol{p}$ is limited by the amplitude/strength of its contribution to the latent hologram, and determined by the following factors:

- Intensity of the indirect illumination contribution from the Virtual Source, given by $|\mathcal{U}_{\text{ill}}(\boldsymbol{p};\bar{\nu})|^2$.
- Albedo of the obscured object $B_o(\boldsymbol{p};\bar{\nu})$.
- Number of speckle cells in the indirect imager PSF $h_{vd}(\boldsymbol{x};\boldsymbol{p},\bar{\nu})$ that can be accommodated within a single detector pixel. This number should not be large (< 100) to avoid amplitude/signal fading due to coherent averaging of speckle amplitudes within a detector pixel [4].

- Radiometric fall-off due to propagation from the Virtual Source to the obscured object point $\boldsymbol{p}$ (encapsulated in the definition of $\mathcal{U}_{\text{ill}}(\boldsymbol{p};\bar{\nu})$), and propagation from the obscured object point $\boldsymbol{p}$ to the $\boldsymbol{n}^{th}$ Virtual Detector pixel (encapsulated in the definition of $h_{vd}(\boldsymbol{x};\boldsymbol{p},\bar{\nu})$).

In practice, the recovery of the latent hologram at the synthetic wavelength is complicated by the presence of the parasitic interference term in the computationally assembled hologram of Eq.(32). Insight into isolating the contributions of this term can be gleaned by examining the exact expression for the parasitic interference component, which is furnished below:

$$\mathcal{U}_{\text{parasitic}}[\boldsymbol{n};\Delta\nu] = \left(\left(\frac{\bar{\nu}+\Delta\nu}{\bar{\nu}}\right)^4\left(\frac{N}{\nu_b}\right)^2 I_r[\boldsymbol{n};\bar{\nu}]\right)\exp(i\phi[\boldsymbol{n};\Delta\nu]) \iint_{\boldsymbol{p}\neq\acute{\boldsymbol{p}}} d\boldsymbol{p}\,d\acute{\boldsymbol{p}} \left\{\begin{matrix}\left(\begin{matrix}\mathcal{U}_{\text{ill}}(\boldsymbol{p};\bar{\nu})\mathcal{U}_{\text{ill}}^*(\acute{\boldsymbol{p}};\bar{\nu}) \\ \times\sqrt{B_o(\boldsymbol{p};\bar{\nu})B_o(\acute{\boldsymbol{p}};\bar{\nu})}\end{matrix}\right)\left(\iint_{(\boldsymbol{n}-0.5F)\Delta}^{(\boldsymbol{n}+0.5F)\Delta} d\boldsymbol{x}\,d\acute{\boldsymbol{x}}\left(\begin{matrix}h_{vd}(\boldsymbol{x};\boldsymbol{p},\bar{\nu}) \\ \times\ h_{vd}^*(\acute{\boldsymbol{x}};\acute{\boldsymbol{p}},\bar{\nu})\end{matrix}\right)\right) \\ \exp\left(i\frac{\Delta\nu}{c}\left(\|\bar{\boldsymbol{s}}-\boldsymbol{p}\| + \left\|\boldsymbol{p}-\begin{bmatrix}-z_d^{-1}\bar{w}_3\boldsymbol{n}\Delta \\ \bar{w}_3\end{bmatrix}\right\|\right)\right)\end{matrix}\right\} \quad (35)$$

It is observed that the product of the indirect imager PSF's for distinct object positions exhibits spatial fluctuations at a scale determined by the numerical aperture of the imaging optics, which is far smaller than the synthetic wavelength. Consequently, the contributions of the parasitic interference term can be suppressed by low-pass filtering the computationally assembled hologram $\mathcal{U}_\Delta[\boldsymbol{n},\bar{\nu}]\times\mathcal{U}_\Delta^*[\boldsymbol{n},\bar{\nu}+\Delta\nu]$ with a cutoff frequency of $\frac{\Delta\nu}{c}$ cycles/meter. The exact same behavior may alternatively be realized by numerical backpropagation of the computational hologram at the synthetic wavelength $\Lambda = c\Delta\nu^{-1}$ meters.

*Sufficient condition for avoiding wavefront aberration in latent hologram*

The ability to recover a latent hologram of the obscured objects by computational mixing of optical holograms recorded at two closely spaced frequencies is predicated on the validity of approximations A5 and A7. Violation of the assumptions (Eqs.(20) and (27)) underlying these approximations induces wavefront aberrations in the latent hologram. Wavefront aberrations in the latent hologram may be avoided by summing up the constraints of Eqs.(20) and (27), namely:

***Rayleigh criterion for wavefront reconstruction by computational mixing of scattered fields at two optical frequencies***

$$\left(\sqrt{\left(\frac{\emptyset_{vs}}{2}\right)^2+\sigma_h^2} + \sqrt{\left(\frac{z_d^{-1}\bar{w}_3F\Delta}{2}\right)^2+\sigma_h^2}\right) < \frac{c\Delta\nu^{-1}}{4} \quad (36)$$

The term $\emptyset_{vs}$ represents the diameter of the beam incident on the Virtual Source surface, while $z_d^{-1}\bar{w}_3F\Delta$ represents the physical extent of the active area of a Virtual Detector pixel. The term $\sigma_h$ represents the RMS roughness of the Virtual Source/Detector surfaces. It is worth noting that the right hand side of Eq.(36) mirrors the Rayleigh quarter wave criterion for the synthetic wavelength, in what can only be described as a serendipitous confluence of constraints.

The inequality of Eq.(36) also divulges a complex tradeoff between the synthetic wavelength $\Lambda = c\Delta\nu^{-1}$ and the Indirect Imaging system parameters namely: the spatial extent of the Virtual Source, the size of a Virtual Detector pixel, and the RMS roughness $\sigma_h$ of the Virtual Source/Detector surfaces. It is observed that smaller Virtual Source diameters, smaller Virtual Detector pixels and smoother Virtual Source/Detector surfaces permit the use of a smaller synthetic wavelength, a fact borne out in experiments.

Furthermore, the inequality of Eq.(36) may be recast to obtain a bound on the largest change in optical frequency $\Delta\nu$, and thereby the smallest synthetic wavelength $\Lambda = c\Delta\nu^{-1}$ that is free of wavefront aberration. The resulting expression is shown below:

$$\Lambda \stackrel{\text{def}}{=} c\Delta\nu^{-1} > 4\left(\sqrt{\left(\frac{\emptyset_{vs}}{2}\right)^2 + \sigma_h^2} + \sqrt{\left(\frac{z_d^{-1}\overline{w}_3 F\Delta}{2}\right)^2 + \sigma_h^2}\right) \tag{37}$$

It is evident from the above discussion that computational mixing of scattered optical field recorded at two closely spaced frequencies $\nu_1 = \bar{\nu}, \nu_2 = (\bar{\nu} + \Delta\nu)$ preserves phase information at scales smaller than the difference frequency $\Delta\nu$, provided the maximum change in path length induced by a change in the optical frequency of interrrogation is smaller than the Rayleigh criterion $\frac{c\Delta\nu^{-1}}{4}$ meters. (***Observation-4***)

## *1.7 Resolution limits*

In the absence of wavefront aberrations, the resolving power of the latent hologram is fundamentally limited by the synthetic wavelength $\Lambda = c\Delta\nu^{-1}$ meters, where $\Delta\nu$ is spacing between the optical frequencies used to interrogate the hidden volume. This limit stems from the inability to reproduce spatial detail exceeding $\Lambda^{-1} = c^{-1}\Delta\nu$ cycles/meter, when replaying the latent hologram. In practice, the achievable lateral resolution is further limited by the spatial extent of the Virtual Detector, and scales inversely with the propagation distance. The behavior is fully consistent with established limits in classical holography [8]. The expression for the lateral resolution at a nominal backpropagation distance of $Z$ meters from the Virtual Detector surface is given by $\Lambda\left(\frac{Z}{M\times(z_d^{-1}\overline{w}_3\Delta)}\right)$. The product term $M\Delta$ represents the physical dimension of the image sensor, which is assumed to be square for simplicity. The product term $z_d^{-1}\overline{w}_3$ represents the transverse magnificaton of the optics used to image the Virtual Detector surface. Consequently, $M \times (z_d^{-1}\overline{w}_3\Delta)$ represents the spatial extent of the Virtual Detector.

*Space-bandwidth product (SBP) of latent hologram*

The finite spatial extent of the latent hologram (given by $M \times (z_d^{-1}\overline{w}_3\Delta)$ meters) combined with the finite spatial frequency bandwidth (given by $2\Lambda^{-1} = 2c^{-1}\Delta\nu$ cycles/meter) of the latent hologram, imposes a hard limit on the complexity of obscured objects that can be faithfully recorded and reproduced. Their product is a measure of the number of degrees of freedom of the latent hologram, and is referred to as the Space-Bandwidth Product (SBP) [3],[9] in optics litearture. The SBP of an optical signal is a measure of its information carrying capacity, and provides an upper bound on system performance. The SBP of the latent hologram is disclosed below:

$$SBP(\mathcal{U}_{\text{latent}}) \stackrel{\text{def}}{=} \left(\left(M \times (z_d^{-1}\overline{w}_3\Delta)\right)\right) \times (2\Lambda^{-1}) \tag{38}$$

The product term $M\Delta$ represents the physical dimension of the image sensor, which is assumed to be square for simplicity. The product term $z_d^{-1}\overline{w}_3$ represents the transverse magnificaton of the optics used to image the Virtual Detector surface. The expression for SBP disclosed in Eq.(38) , is strictly valid when the recovered latent hologram is devoid of any wavefront aberration at the synthetic wavelength. The expression for the smallest synthetic wavelength that is devoid of wavefront aberration was first disclosed in Eq.(37). sufficient condition for avoiding wavefront errors in the latent hologram. Incorporating the aformentioned result into the expression for the SBP, yields an upper-bound on the SBP of the latent hologram:

***Upper-bound of SBP of Indirect Imaging using Synthetic Wavelength Holography***

$$SBP \leq \frac{\left(M \times (z_d^{-1}\overline{w}_3\Delta)\right)}{2\left(\sqrt{\left(\frac{\emptyset_{vs}}{2}\right)^2 + \sigma_h^2} + \sqrt{\left(\frac{z_d^{-1}\overline{w}_3 F\Delta}{2}\right)^2 + \sigma_h^2}\right)} \tag{39}$$

The term $\emptyset_{vs}$ represents the diameter of the beam incident on the Virtual Source surface, while $z_d^{-1}\bar{w}_3\Delta$ and $z_d^{-1}\bar{w}_3 F\Delta$ represents the active area and pixel pitch of a Virtual Detector pixel, respectively. The term $\sigma_h$ represents the RMS roughness of the Virtual Source/Detector surfaces. It is worth noting that the expression for SBP disclosed in Eq.(39), closely resembles Eq.(6) of the main manuscript. The term in the denominator may be viewed as a proxy for the peak-valley wavefront aberration at the synthetic wavelength $\Lambda$.

The upper bound on SBP for Synthetic Wavelength Holography disclosed in Eq.(39) is by no means the best that can be achieved from a theoretical standpoint. The asymptotic limit of the SBP for Indirect Imaging using Synthetic Wavelength Holography is obtained as $F \to 1$, $\emptyset_{vs} \to c\bar{\nu}^{-1}$ and $z_d^{-1}\bar{w}_3 F\Delta \to 0.5c\bar{\nu}^{-1}$. These system parameters represent the absolute best that can achieved from the standpoint of sensor fill factor, spot diameter of the Virtual Source and recording fields with the highest resolution using classical optics. Under these restrictions, the RMS roughness of the intermediary surface $\sigma_h \gg \emptyset_{vs}, z_d^{-1}\bar{w}_3 F\Delta$ so that the asymptotic SBP is given by:

$$SBP < (Mc\bar{\nu}^{-1})\left(\frac{1}{4\sigma_h}\right) \quad (40)$$

Consequently, the information carrying capacity of Synthetic Wavelength Holography is fundamentally limited by the roughness of the intermediary scattering surfaces that are adapted to serve as the Virtual Source/Detector. A comparison of the definition of the Space-Bandwdth product, disclosed in Eq(38), and the expression for the asymptotic SBP disclosed in Eq.(40), reveals a fundamental limit to the achievable resolution in Synthetic Wavelength Holography, and is given by $\Lambda > 8\sigma_h$.

*Localization accuracy of the latent hologram*

In the absence of wavefront aberrations, the longitudinal resolution of the latent hologram is limited to $2\Lambda\left(\frac{Z}{M\times(z_d^{-1}\bar{w}_3\Delta)}\right)^2$, and fully consistent with established limits in classical holography [8]. This limits our ability to precisely localize obscured objects within the hidden volume, and its impact is best illustrated in Figure-5 of the main manuscript. The traditional approach to tackling this problem is time-resolved holography using pulsed sources. Unfortunately, pulsed sources lack the temporal coherence needed to record holograms of objects obscured from view. The problem may be remedied by examining a computational approach to synthesizing light pulses using a multitude of optical frequencies, and is the topic of Section-2.

## 2. *Optical sectioning using a multitude of regularly spaced frequencies*

It is common knowledge that an ultrashort pulse train admits a Fourier series decomposition in the optical frequency domain. Herein we seek to computationally mimic the behavior by independently interrogating the hidden scene using a countably finite number of regularly spaced optical frequencies, and record the corresponding holograms. By computationally delaying the hologram recorded at each optical frequency, and accumulating the result across optical frequencies, it is possible to mimic interogation of the hidden scene by a pulse train. The process is illustrated in **Figure3**, and is inspired by work in Fourier Synthesis Holography [10], and holographic laser radar [11],[12].

The periodicity of the pulse train is determined by the smallest separation between the optical frequencies, while the pulse duration is determined by the largest separation between the optical frequencies. It can be shown that $K$ optical frequencies spaced apart by $\Delta\nu$ Hz can be used to computationally synthesize a periodic optical pulse train, with pulse duration $\tau_p = (K\Delta\nu)^{-1}$and repetition rate $\tau_{\text{rep}} = \Delta\nu^{-1}$ seconds. The shape of the pulse may be manipulated by appropriately weighting the holograms recorded at each optical frequency, prior to accumulation. In the simple case that the weights are chosen uniformly, the pulse envelope resembles a sinc-like function. By additionally delaying the

hologram at each optical frequency, it is possible to synthesize a delayed pulse train that preferentially selects ray paths from the Virtual Source to the Virtual Detector with a prescribed round-trip distance. The notion is illustrated in the gary box designated "Computational path-length filtering" in **Figure3**.

Unfortunately, the computationally filtered hologram $\mathcal{U}_{\text{fltrd}}[\boldsymbol{n}]$ is still plagued by speckle at the optical frequency. The problem is remedied by computationally mixing the filtered hologram with the hologram recorded at the optical frequency $\bar{\nu}$. The expression for the resulting latent hologram closely resembles the expression for the two frequency latent hologram disclosed in Eq.(34). The distinction emerges in the additional attenuation introduced by the path length filter $g\left(\|\bar{\boldsymbol{s}}-\boldsymbol{p}\|+\left\|\boldsymbol{p}-\begin{bmatrix}-z_d^{-1}\bar{w}_3\boldsymbol{n}\Delta\\ \bar{w}_3\end{bmatrix}\right\|-D\right)$. This filter promotes constructive interference of light at the synthetic wavelength for select propagation distances, and promotes destructive interference at remaining propagation distances.

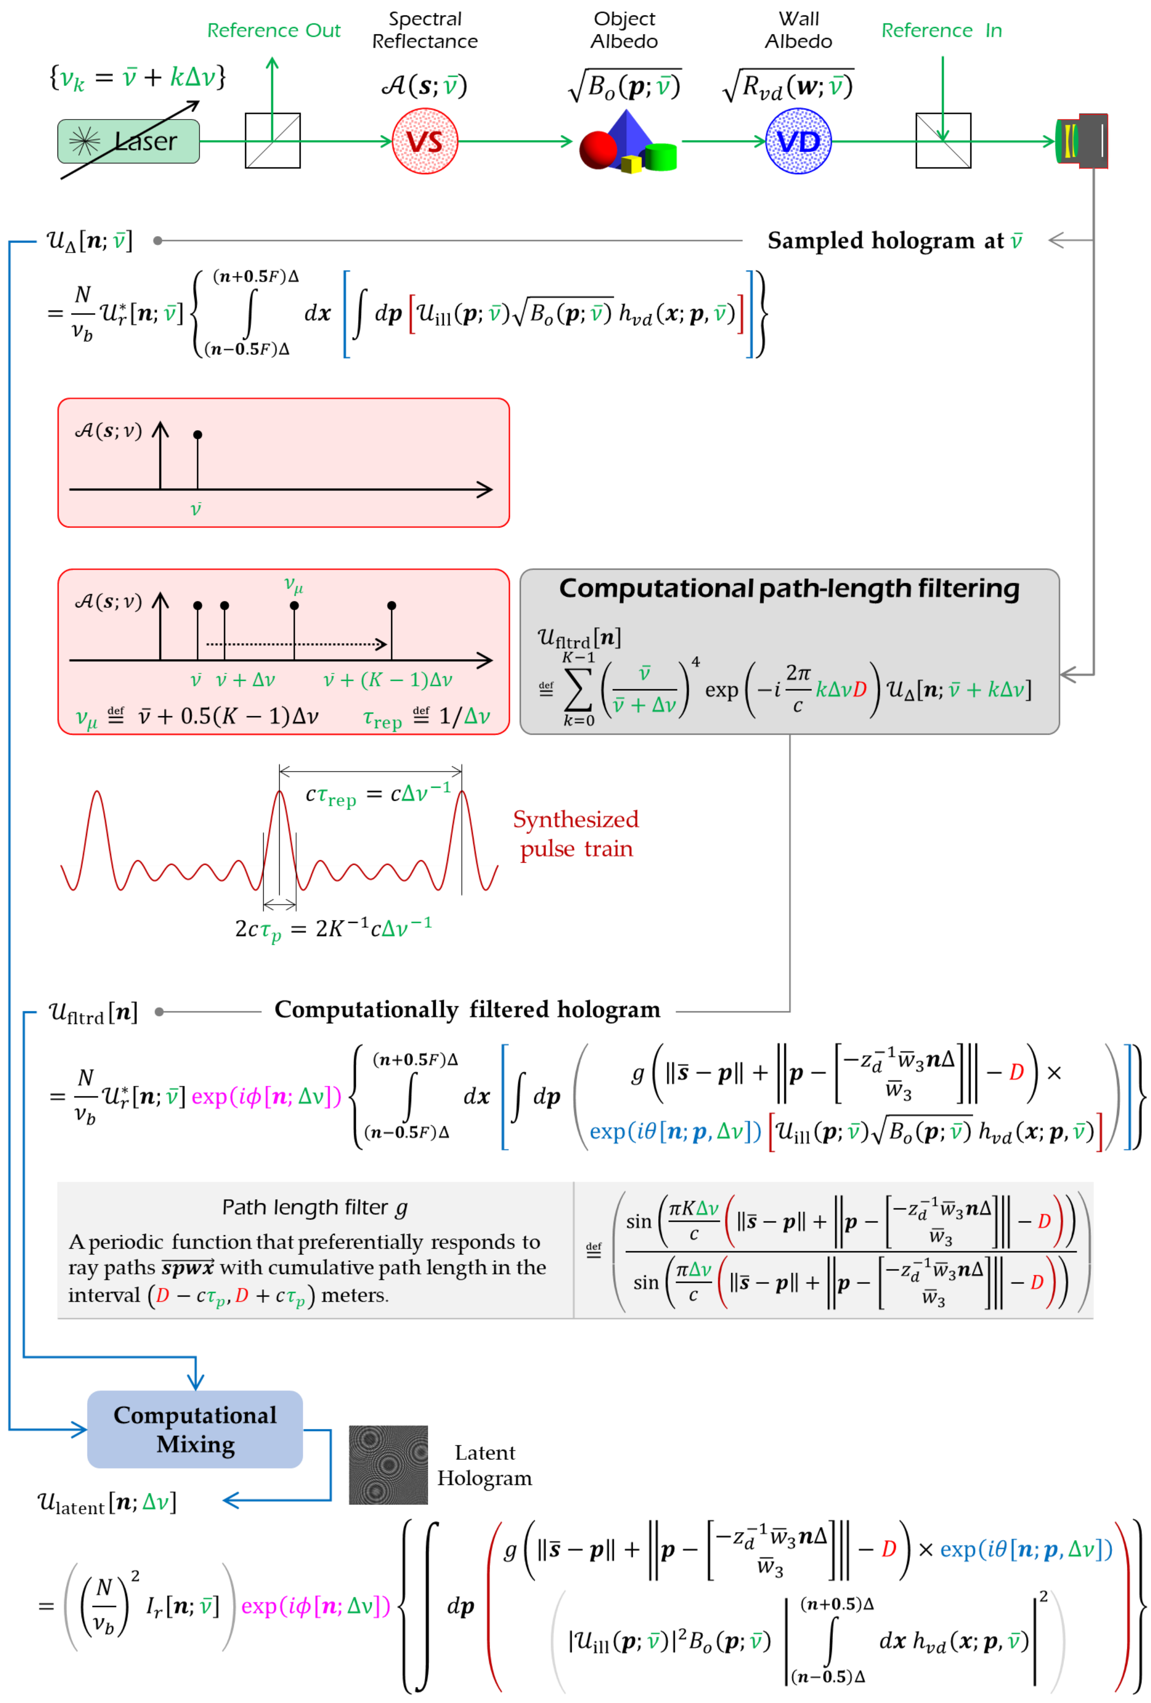


**Figure3:** Optical sectioning using a multitude of regularly spaced frequencies

The periodicity of the synthesized pulse train introduces periodic ambiguites in the response of the path length filter. This fact is corroborated in the experimental results of Figure-5 furnished in the main manuscript.

The latent hologram assembled using the proposed approach is insensitive to scattering at the Virtual Source and Virtual Detector, features a lateral resolution limit of $c\left(\frac{(K-1)}{2}\Delta\nu\right)^{-1}$ meters and a longitudinal resolution of $2c(K\Delta\nu)^{-1}$ meters.

## 3. *Relating the optical blur at $\bar{\nu}+\Delta\nu$ to the optical blur at $\bar{\nu}$*

The optical blur associated with imaging the VD surface may be modeled as a paraxial blur [3] with image side numerical aperture $Dz_d^{-1}$, where $D$ is the exit pupil diameter. The resulting amplitude PSF was originally disclosed in Eq.(2), and repeated below for the benefit of the reader.

$$h_{\text{blur}}\left(\boldsymbol{x} \overset{\text{def}}{=} \begin{bmatrix} x_1 \\ x_2 \end{bmatrix}; \boldsymbol{w} \overset{\text{def}}{=} \begin{bmatrix} w_1 \\ w_2 \\ w_3 \end{bmatrix}, \bar{\nu}\right) = \left(\begin{matrix} \left(\frac{\bar{\nu}}{ic}\right)^2 \frac{1}{z_d w_3} \exp\left(i\frac{2\pi\bar{\nu}}{c}\left[z_d + w_3 + \frac{[x_1^2+x_2^2]}{2z_d} + \frac{[w_1^2+w_2^2]}{2w_3}\right]\right) \\ \int dudv \left[P(u,v)\exp\left(i\frac{2\pi\bar{\nu}}{c}\left[\frac{1}{z_d}+\frac{1}{w_3}-\frac{1}{f}\right](u^2+v^2)\right)\exp\left(-i\frac{2\pi\bar{\nu}}{c}\left(\left[\frac{x_1}{z_d}+\frac{w_1}{w_3}\right]u + \left[\frac{x_2}{z_d}+\frac{w_2}{w_3}\right]v\right)\right)\right] \end{matrix}\right) \tag{41}$$

The term $P(u,v)$ represents the transmittance function of the exit pupil and modeled as an indicator function with diameter $D$. The term $f$ represents the focal length of the imaging optic. The depth $w_3$ of a point on the VD surface is measured with respect to the entrance pupil plane of the imaging optic.

The expression for the optical blur resulting from a small change in the optical frequency of the CW illumination source is disclosed below:

$$\begin{aligned} &h_{\text{blur}}\left(\boldsymbol{x} \overset{\text{def}}{=} \begin{bmatrix} x_1 \\ x_2 \end{bmatrix}; \boldsymbol{w} \overset{\text{def}}{=} \begin{bmatrix} w_1 \\ w_2 \\ w_3 \end{bmatrix}, \bar{\nu}+\Delta\nu\right) \\ &= \left(\begin{matrix} \left(\frac{\bar{\nu}+\Delta\nu}{ic}\right)^2 \frac{1}{z_d w_3}\exp\left(i2\pi\frac{(\bar{\nu}+\Delta\nu)}{c}\left[z_d + w_3 + \frac{[x_1^2+x_2^2]}{2z_d} + \frac{[w_1^2+w_2^2]}{2w_3}\right]\right) \\ \int dudv\left[P(u,v)\exp\left(i2\pi\frac{(\bar{\nu}+\Delta\nu)}{c}\left[\frac{1}{z_d}+\frac{1}{w_3}-\frac{1}{f}\right](u^2+v^2)\right)\exp\left(-i2\pi\frac{(\bar{\nu}+\Delta\nu)}{c}\left(\left[\frac{x_1}{z_d}+\frac{w_1}{w_3}\right]u+\left[\frac{x_2}{z_d}+\frac{w_2}{w_3}\right]v\right)\right)\right]\end{matrix}\right) \\ &= \left(\begin{matrix} \left(\begin{matrix} \left\{\left(\frac{\bar{\nu}+\Delta\nu}{\bar{\nu}}\right)^2 \exp\left(i2\pi\frac{\Delta\nu}{c}\left[z_d + \frac{[x_1^2+x_2^2]}{2z_d} + w_3 + \frac{[w_1^2+w_2^2]}{2w_3}\right]\right)\right\} \times \\ \left\{\left(\frac{\bar{\nu}}{ic}\right)^2 \frac{1}{z_d w_3}\exp\left(i2\pi\frac{(\bar{\nu}+\Delta\nu)}{c}\left[z_d + w_3 + \frac{[x_1^2+x_2^2]}{2z_d} + \frac{[w_1^2+w_2^2]}{2w_3}\right]\right)\right\} \end{matrix}\right) \times \\ \left(\begin{matrix} \left\{\int dudv\left[P(u,v)\exp\left(i2\pi\frac{\bar{\nu}}{c}\left[\frac{1}{z_d}+\frac{1}{w_3}-\frac{1}{f}\right](u^2+v^2)\right)\exp\left(-i2\pi\frac{\bar{\nu}}{c}\left(\left[\frac{x_1}{z_d}+\frac{w_1}{w_3}\right]u+\left[\frac{x_2}{z_d}+\frac{w_2}{w_3}\right]v\right)\right)\right]\right\} \otimes \\ \left\{\int dudv\left[\exp\left(i2\pi\frac{\Delta\nu}{c}\left[\frac{1}{z_d}+\frac{1}{w_3}-\frac{1}{f}\right](u^2+v^2)\right)\exp\left(-i2\pi\frac{\Delta\nu}{c}\left(\left[\frac{x_1}{z_d}+\frac{w_1}{w_3}\right]u+\left[\frac{x_2}{z_d}+\frac{w_2}{w_3}\right]v\right)\right)\right]\right\} \end{matrix}\right) \end{matrix}\right) \end{aligned} \tag{42}$$

***Observation-4:*** The defocus aberration $\exp\left(i\frac{2\pi\Delta\nu}{c}\left[\frac{1}{z_d}+\frac{1}{w_3}-\frac{1}{f}\right](u^2+v^2)\right)$ induced by a small change in the optical frequency can be omitted so long as $\left[\frac{1}{z_d}+\frac{1}{w_3}-\frac{1}{f}\right]\frac{\Delta\nu}{c} \ll \frac{1}{2\pi}$. This implies that the defocus in waves $< \frac{1}{8^{\text{th}}}$ the synthetic wavelength $c\Delta\nu^{-1}$ meters.

Incorporating the aforementioned constraint into Eq.(42) yields the revised expressions for optical blur disclosed in Eqs.(43)-(44)

$$h_{\text{blur}}\left(\boldsymbol{x} \stackrel{\text{def}}{=} \begin{bmatrix} x_1 \\ x_2 \end{bmatrix}; \boldsymbol{w} \stackrel{\text{def}}{=} \begin{bmatrix} w_1 \\ w_2 \\ w_3 \end{bmatrix}, \bar{\nu} + \Delta\nu\right)$$
$$= \left( \begin{matrix} \left( \begin{matrix} \left\{ \left(\frac{\bar{\nu}+\Delta\nu}{\bar{\nu}}\right)^2 \exp\left(i2\pi\frac{\Delta\nu}{c}\left[z_d + \frac{[x_1^2+x_2^2]}{2z_d} + w_3 + \frac{[w_1^2+w_2^2]}{2w_3}\right]\right)\right\} \times \\ \left\{ \left(\frac{\bar{\nu}}{ic}\right)^2 \frac{1}{z_d w_3} \exp\left(i2\pi\frac{(\bar{\nu}+\Delta\nu)}{c}\left[z_d + w_3 + \frac{[x_1^2+x_2^2]}{2z_d} + \frac{[w_1^2+w_2^2]}{2w_3}\right]\right)\right\} \end{matrix} \right) \times \\ \left( \begin{matrix} \left\{ \int dudv \left[ P(u,v) \exp\left(i2\pi\frac{\bar{\nu}}{c}\left[\frac{1}{z_d}+\frac{1}{w_3}-\frac{1}{f}\right](u^2+v^2)\right) \exp\left(-i2\pi\frac{\bar{\nu}}{c}\left(\left[\frac{x_1}{z_d}+\frac{w_1}{w_3}\right]u + \left[\frac{x_2}{z_d}+\frac{w_2}{w_3}\right]v\right)\right)\right]\right\} \otimes \\ \left\{ \int dudv \exp\left(-i2\pi\frac{\Delta\nu}{c}\left(\left[\frac{x_1}{z_d}+\frac{w_1}{w_3}\right]u + \left[\frac{x_2}{z_d}+\frac{w_2}{w_3}\right]v\right)\right)\right\} \end{matrix} \right) \end{matrix} \right) \tag{43}$$

$$h_{\text{blur}}\left(\boldsymbol{x} \stackrel{\text{def}}{=} \begin{bmatrix} x_1 \\ x_2 \end{bmatrix}; \boldsymbol{w} \stackrel{\text{def}}{=} \begin{bmatrix} w_1 \\ w_2 \\ w_3 \end{bmatrix}, \bar{\nu} + \Delta\nu\right)$$
$$= \left( \begin{matrix} \left( \begin{matrix} \left\{ \left(\frac{\bar{\nu}+\Delta\nu}{\bar{\nu}}\right)^2 \exp\left(i2\pi\frac{\Delta\nu}{c}\left[z_d + \frac{[x_1^2+x_2^2]}{2z_d} + w_3 + \frac{[w_1^2+w_2^2]}{2w_3}\right]\right)\right\} \times \\ \left\{ \left(\frac{\bar{\nu}}{ic}\right)^2 \frac{1}{z_d w_3} \exp\left(i2\pi\frac{(\bar{\nu}+\Delta\nu)}{c}\left[z_d + w_3 + \frac{[x_1^2+x_2^2]}{2z_d} + \frac{[w_1^2+w_2^2]}{2w_3}\right]\right)\right\} \end{matrix} \right) \times \\ \left( \begin{matrix} \left\{ \int dudv \left[ P(u,v) \exp\left(i2\pi\frac{\bar{\nu}}{c}\left[\frac{1}{z_d}+\frac{1}{w_3}-\frac{1}{f}\right](u^2+v^2)\right) \exp\left(-i2\pi\frac{\bar{\nu}}{c}\left(\left[\frac{x_1}{z_d}+\frac{w_1}{w_3}\right]u + \left[\frac{x_2}{z_d}+\frac{w_2}{w_3}\right]v\right)\right)\right]\right\} \otimes \\ \left\{ \delta\left(\frac{\Delta\nu}{c}\left[\frac{x_1}{z_d}+\frac{w_1}{w_3}\right]u, \frac{\Delta\nu}{c}\left[\frac{x_2}{z_d}+\frac{w_2}{w_3}\right]v\right)\right\} \end{matrix} \right) \end{matrix} \right) \tag{44}$$

The Dirac-delta function in Eq.(44) is a restatement of the imaging identity: $x_1 = -z_d \frac{w_1}{w_3}, x_2 = -z_d \frac{w_2}{w_3}$ first disclosed in Eq.(1), and is intrinsic to the process of imaging the Virtual Detector surface. The integral highlighted in blue yields a function of the form $g\left(\frac{\bar{\nu}}{c}\left(\left[\frac{x_1}{z_d}+\frac{w_1}{w_3}\right], \frac{\bar{\nu}}{c}\left[\frac{x_2}{z_d}+\frac{w_2}{w_3}\right]\right)\right)$, which when convolved with the the Dirac-delta function remains unchanged in functional form. This behavior can be attributed to the fact that the centroid of the optical blur spot $h_{\text{blur}}(\boldsymbol{x}; \boldsymbol{w}, \bar{\nu})$ also satifies the imaging identity. In view of this relation, the Dirac-delta function can be ignored from subsequent analysis. Consequently,

$$h_{\text{blur}}\left(\boldsymbol{x} \stackrel{\text{def}}{=} \begin{bmatrix} x_1 \\ x_2 \end{bmatrix}; \boldsymbol{w} \stackrel{\text{def}}{=} \begin{bmatrix} w_1 \\ w_2 \\ w_3 \end{bmatrix}, \bar{\nu} + \Delta\nu\right)$$
$$= \left(\frac{\bar{\nu}+\Delta\nu}{\bar{\nu}}\right)^2 \left[\exp\left(i2\pi\frac{\Delta\nu}{c}\left[z_d + \frac{[x_1^2+x_2^2]}{2z_d} + w_3 + \frac{[w_1^2+w_2^2]}{2w_3}\right]\right)\right] h_{\text{blur}}\left(\boldsymbol{x} \stackrel{\text{def}}{=} \begin{bmatrix} x_1 \\ x_2 \end{bmatrix}; \boldsymbol{w} \stackrel{\text{def}}{=} \begin{bmatrix} w_1 \\ w_2 \\ w_3 \end{bmatrix}, \bar{\nu}\right) \tag{45}$$

Further simplification is possible if it is assumed that the RMS roughness of the VD surface is much smaller than the mean depth of the Virtual Detector surface, so that

$$\frac{1}{w_3} \approx \frac{1}{\bar{w}_3} - \left(\frac{\delta w_3}{\bar{w}_3^2}\right) \tag{46}$$

where the depth $w_3$ of a point on the Virtual Detector surface is assumed to be a 2D random variable with mean value $\bar{w}_3$ and a zero-mean stochastic term $\delta w_3$ representing the surface height fluctuations. If additionally the peak height fluctuation in the VD surface $\frac{\delta w_3}{\bar{w}_3} < \frac{c(\Delta\nu)^{-1}}{8} \bar{w}_3$, then the linear phase fluctuation $\frac{2\pi\Delta\nu}{c} \frac{\delta w_3}{\bar{w}_3^2}$ induced by the optical roughness of the Virtual Detector surface may be omitted from further consideration. Incorporating the above into Eqs.(45)-(46) yields the following simplified relation between the optical blurs at $\bar{\nu}, \bar{\nu} + \Delta\nu$:

$$h_{\text{blur}}\left(\boldsymbol{x} \stackrel{\text{def}}{=} \begin{bmatrix} x_1 \\ x_2 \end{bmatrix}; \boldsymbol{w} \stackrel{\text{def}}{=} \begin{bmatrix} w_1 \\ w_2 \\ w_3 \end{bmatrix}, \bar{\nu} + \Delta\nu\right)$$
$$= \left(\frac{\bar{\nu} + \Delta\nu}{\bar{\nu}}\right)^2 \left[\exp\left(i2\pi\frac{\Delta\nu}{c}\left[z_d + \frac{[x_1^2 + x_2^2]}{2z_d} + \bar{w}_3 + \frac{[w_1^2 + w_2^2]}{2\bar{w}_3}\right]\right)\right] h_{\text{blur}}\left(\boldsymbol{x} \stackrel{\text{def}}{=} \begin{bmatrix} x_1 \\ x_2 \end{bmatrix}; \boldsymbol{w} \stackrel{\text{def}}{=} \begin{bmatrix} w_1 \\ w_2 \\ w_3 \end{bmatrix}, \bar{\nu}\right) \quad (47)$$

This concludes the proof.

## 4. *Spectral correlations in volumetric scatter*

The existence of spectral correlations in scattered light is central to our efforts to mitigating the effects of scattering, using the principles of Synthetic Wavelength Holography. The present section seeks to experimentally establish the existence of spectral field correlations in the wavefronts emerging from a thin volumetric scattering sample. Details of the experimental apparatus used to record the scattered wavefronts are available in Kadobianskyi et.al. [13]. The authors of this work sought to characterize the spatio-temporal response of a tvolumetric scattering sample (thickness $L = 360\,\mu m, 720\mu m$, scattering mean free path $\ell = 90\mu m$), by recording scattered monochromatic wavefronts for 801 equally spaced optical frequencies in the $690nm$ to $940nm$ range. It was observed that the recorded monochromatic speckle fields exhibit unknown residual phase variations, due to factors such as dispersion, chromatic focus shift, and reference beam phase drift. Such phase variations can be readily discerned by computationally assembling holograms at the synthetic wavelength. The process is illustrated in Figure4. The image insets 4(a-b),4(d-e) illustrate the randomized dephasing of scattered light at two neighboring wavelengths $\lambda_1 = c\bar{\nu}, \lambda_2 = c(\bar{\nu} + \Delta\nu)$, characterized by a fixed frequency separation of $\Delta\nu = 144.54\,GHz$. A synthetic wavelength hologram is computationally assembled by mixing the speckle fields $\mathcal{U}(\boldsymbol{x}; \bar{\nu}) \times \mathcal{U}^*(\boldsymbol{x}; \bar{\nu} + \Delta\nu)$. The phase of the synthetic wavelength hologram (image insets 4(c),4(f)) exhibits a weak carrier artifact consistent with the observation of interference fringes due to inter-reflections between the laser aperture and a polarized beamsplitter in the illumination path; according to the authors of [13]. Figure5 demonstrates the same result for a second scattering sample that is twice as thick as the sample used used in Figure4.

Although the goal of work by Kadobianskyi et.al. [13]. is markedly different different from our goal of mitigating scatter, both approaches exploit spectral correlations in the scattered wavefronts. The experimental results furnished in Figures-4 and 5 serve to corroborate the generality of the principles underlying Synthetic Wavelength Holography, and its utility in recovering phase information from scattered wavefronts recorded at optical wavelengths.

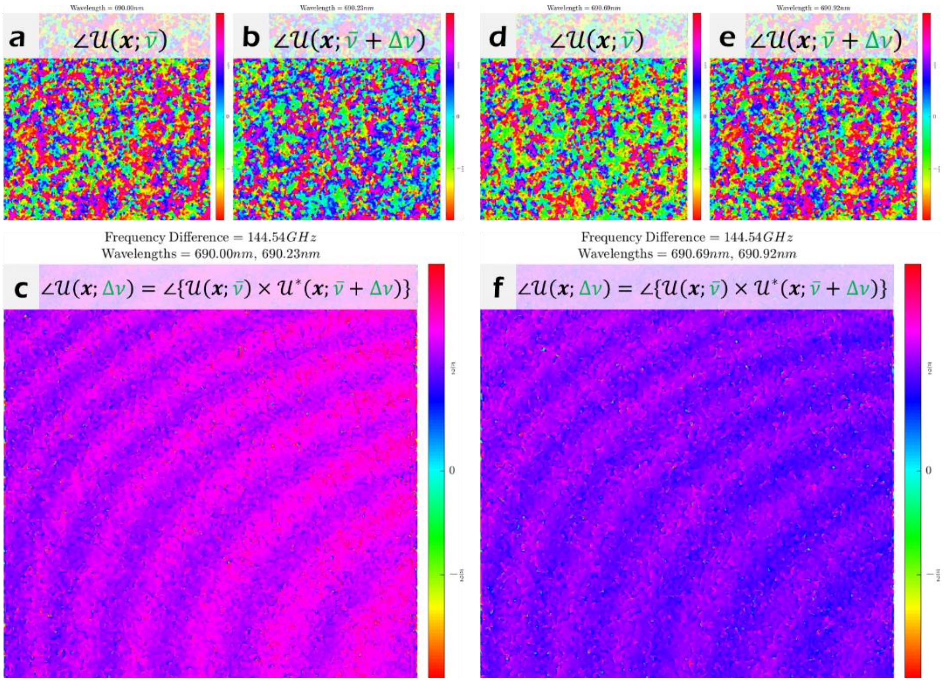


**Figure4:** Spectral correlations in the scattered wavefronts emerging from a thin volumetric scattering sample (thickness $L = 360\mu m$, scattering mean free path $\ell = 90\mu m$)

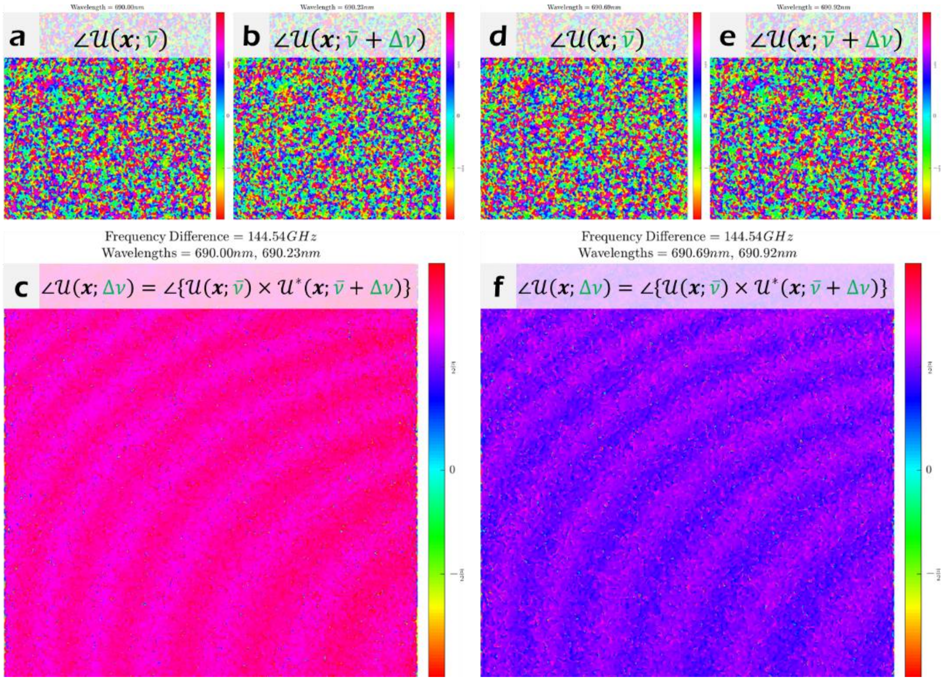


**Figure5:** Spectral correlations in the scattered wavefronts emerging from a thin volumetric scattering sample (thickness $L = 720\mu m$, scattering mean free path $\ell = 90\mu m$)

### *References*


[1] Goodman JW. Speckle phenomena in optics: theory and applications. Roberts and Company Publishers; 2007.

[2] Heliotis Helicam C3 Manual (http://www.heliotis.ch/html/heliDocumentation.htm).

[3] J. W. Goodman, Introduction to Fourier Optics, McGraw-Hill, New York, NY, USA, 2ed edition, 1996.

[4] Aniceto Belmonte, "Statistical model for fading return signals in coherent lidars," Appl. Opt. 49, 6737-6748 (2010)

[5] Madabhushi, Balaji. "Indirect Imaging using Heterodyne Remote Digital Holography." MS thesis., SOUTHERN METHODIST UNIVERSITY, 2018.

[6] Liu, Y., Shen, Y., Ma, C., Shi, J., & Wang, L. V. (2016). Lock-in camera based heterodyne holography for ultrasound-modulated optical tomography inside dynamic scattering media. Applied physics letters, 108(23), 231106. doi:10.1063/1.4953630

[7] A. W. Lohmann and D. P. Paris, "Space-Variant Image Formation*," J. Opt. Soc. Am. 55, 1007-1013 (1965)

[8] Tatiana Latychevskaia, "Lateral and axial resolution criteria in incoherent and coherent optics and holography, near- and far-field regimes," Appl. Opt. 58, 3597-3603 (2019)

[9] Adolf W. Lohmann, Rainer G. Dorsch, David Mendlovic, Zeev Zalevsky, and Carlos Ferreira, "Space–bandwidth product of optical signals and systems," J. Opt. Soc. Am. A 13, 470-473 (1996)

[10] E. Arons, D. Dilworth, M. Shih, and P. C. Sun, "Use of Fourier synthesis holography to image through inhomogeneities," Opt. Lett. 18, 1852-1854 (1993)

[11] Joseph C. Marron and Kirk S. Schroeder, "Holographic laser radar," Opt. Lett. 18, 385-387 (1993)

[12] Joseph C. Marron and Kirk S. Schroeder, "Three-dimensional lensless imaging using laser frequency diversity," Appl. Opt. 31, 255-262 (1992)

[13] Mykola Kadobianskyi, Ioannis N. Papadopoulos, Thomas Chaigne, Roarke Horstmeyer, and Benjamin Judkewitz, "Scattering correlations of time-gated light," Optica 5, 389-394 (2018)
